# Supplementary material for: Multiwavelength study of observed and predicted pulsation properties of First overtone Cepheids in the Magellanic Clouds
Source: arXiv:2506.15171 source file (2025-06-18)
Supplement: Supplementary file 1 [file Magellanic_Clouds_fufo_Cepheids_supplementary_data.pdf]

# Multiwavelength study of observed and predicted pulsation properties of First overtone Cepheids in the Magellanic Clouds

Kerdaris Kurbah[1⋆], Shashi M. Kanbur[2†], Sukanta Deb[1,3‡], Anupam Bhardwaj[4], Mami Deka[5], Susmita Das[4,6,7], Gautam Bhuyan[1]

[1]*Department of Physics, Cotton University, Guwahati 781001, Assam, India*
[2]*Department of Physics, State University of New York, Oswego, NY 23126, USA*
[3]*Space and Astronomy Research Center, Cotton University, Guwahati 781001, Assam, India*
[4]*Inter-University Center for Astronomy and Astrophysics (IUCAA), Post Bag 4, Ganeshkhind, Pune 411 007, India*
[5]*INAF-Osservatorio astronomico di Capodimonte, Via Moiariello 16, I-80131 Napoli, Italy*
[6]*Konkoly Observatory, Research Centre for Astronomy and Earth Sciences, HUN-REN, Konkoly-Thege Miklós út 15-17, H-1121, Budapest, Hungary*
[7]*CSFK, MTA Centre of Excellence, Budapest, Konkoly Thege Miklós út 15-17., H-1121, Hungary*

17 June 2025

**ABSTRACT**

We present a detailed analysis of the light curves and pulsation properties of First Overtone (FO) Cepheids in the Magellanic Clouds (MCs) obtained using observations and predictions from stellar pulsation models. Multiwavelength observational light curves were compiled from the literature (OGLE-IV, Gaia and VMC). We investigate the period-amplitude (PA), period-colour (PC), period-luminosity (PL), and amplitude-colour (AC) relations for FO Cepheids at multiwavelengths. We find that the PA distribution of FO Cepheids in the MCs modelled using a Gaussian Mixture Model shows that the SMC consists of higher amplitude stars than the LMC. We find multiple break-points in the PC/PL/AC relations for FO/FU Cepheids in the optical and near-infrared bands including the one near to $P = 2.5$ d in the MCs using piecewise regression analysis and $F$-test statistics. Similarly, for the LMC FO Cepheids, we find a break-point in the PC/PL/AC relations near $P = 0.58$ d.The slopes of the PC relation for LMC FO Cepheids are found to be shallow for $0.58 < P(\mathrm{d}) < 2.5$ but steeper for $P < 0.58$ d and $P > 2.5$ d. We complemented the observed relations using theoretical models for FO Cepheids with chemical compositions $Z = 0.008$ and $Z = 0.004$, appropriate for the LMC and SMC, respectively computed with MESA-RSP. Our results show that the pulsation properties of FO Cepheids in PC/PL/AC relations and colour-magnitude diagram are strongly correlated and their connections can provide stringent constraints for the theoretical pulsation models.

**Key words:** stars: variable: Cepheids-galaxies: Magellanic Clouds-methods: data analysis-methods: statistical

This paper has been typeset from a TEX/LATEX file prepared by the author.

⋆ E-mail: kerdarisbahkur@gmail.com
† E-mail:shashi.kanbur@oswego.edu
‡ E-mail:sukantodeb@gmail.com

© 0000 The Authors

**Table 1.** Coefficients of the empirical PC relation for LMC and SMC FU Cepheids at maximum and minimum light assuming a break at $P = 2.5$ d. The bold-face entries indicates the significance of the break.

| | Phase | $a_{all}$ | $b_{all}$ | $a_s$ | $b_s$ | $a_l$ | $b_l$ | $F$ | $p(F)$ |
|---|---|---|---|---|---|---|---|---|---|
| | | | | | LMC | | | | |
| $V-I$ | Max | 0.362 ± 0.013 | 0.249 ± 0.008 | 0.139 ± 0.067 | 0.325 ± 0.020 | 0.392 ± 0.016 | 0.230 ± 0.010 | 8.009 | **0.000** |
| | Min | 0.237 ± 0.006 | 0.631 ± 0.003 | 0.147 ± 0.031 | 0.656 ± 0.009 | 0.241 ± 0.007 | 0.629 ± 0.004 | 3.992 | **0.018** |
| $V-G$ | Max | 0.196 ± 0.012 | −0.163 ± 0.007 | 0.188 ± 0.099 | −0.106 ± 0.032 | 0.203 ± 0.013 | −0.117 ± 0.008 | 0.349 | 0.705 |
| | Min | 0.086 ± 0.007 | 0.118 ± 0.005 | 0.054 ± 0.044 | 0.130 ± 0.013 | 0.091 ± 0.009 | 0.114 ± 0.005 | 0.677 | 0.508 |
| $V-Rp$ | Max | 0.293 ± 0.027 | 0.140 ± 0.015 | 0.187 ± 0.170 | 0.144 ± 0.053 | 0.243 ± 0.033 | 0.171 ± 0.019 | 4.063 | 0.017 |
| | Min | 0.209 ± 0.024 | 0.668 ± 0.014 | 0.037 ± 0.119 | 0.697 ± 0.037 | 0.182 ± 0.029 | 0.686 ± 0.018 | 3.083 | 0.046 |
| $V-Y$ | Max | 0.623 ± 0.028 | 0.122 ± 0.016 | 0.303 ± 0.156 | 0.234 ± 0.048 | 0.673 ± 0.034 | 0.090 ± 0.020 | 4.369 | **0.012** |
| | Min | 0.261 ± 0.023 | 0.930 ± 0.013 | 0.422 ± 0.111 | 0.860 ± 0.034 | 0.214 ± 0.029 | 0.960 ± 0.017 | 4.134 | **0.016** |
| $V-J$ | Max | 0.684 ± 0.029 | 0.357 ± 0.017 | 0.466 ± 0.154 | 0.456 ± 0.048 | 0.760 ± 0.036 | 0.307 ± 0.022 | 6.305 | **0.000** |
| | Min | 0.360 ± 0.022 | 1.189 ± 0.013 | 0.572 ± 0.122 | 1.117 ± 0.038 | 0.330 ± 0.027 | 1.208 ± 0.017 | 2.654 | 0.070 |
| $V-Ks$ | Max | 0.811 ± 0.029 | 0.635 ± 0.017 | 0.446 ± 0.159 | 0.761 ± 0.049 | 0.865 ± 0.036 | 0.600 ± 0.022 | 4.852 | **0.006** |
| | Min | 0.491 ± 0.018 | 1.508 ± 0.010 | 0.691 ± 0.096 | 1.423 ± 0.029 | 0.435 ± 0.022 | 1.544 ± 0.013 | 9.453 | **0.000** |
| | | | | | SMC | | | | |
| $V-I$ | Max | 0.302 ± 0.011 | 0.271 ± 0.004 | 0.205 ± 0.032 | 0.296 ± 0.007 | 0.532 ± 0.028 | 0.127 ± 0.0181 | 39.210 | **0.000** |
| | Min | 0.162 ± 0.005 | 0.695 ± 0.002 | 0.160 ± 0.016 | 0.695 ± 0.003 | 0.150 ± 0.012 | 0.704 ± 0.007 | 1.120 | 0.326 |
| $V-G$ | Max | 0.185 ± 0.030 | −0.114 ± 0.014 | 0.081 ± 0.134 | −0.088 ± 0.033 | 0.254 ± 0.048 | −0.158 ± 0.030 | 0.957 | **0.000** |
| | Min | 0.050 ± 0.008 | 0.183 ± 0.003 | 0.098 ± 0.030 | 0.170 ± 0.007 | −0.005 ± 0.018 | 0.219 ± 0.011 | 6.208 | **0.000** |
| $V-Rp$ | Max | 0.251 ± 0.030 | 0.250 ± 0.013 | 0.136 ± 0.125 | 0.285 ± 0.031 | 0.454 ± 0.052 | 0.114 ± 0.033 | 8.902 | **0.000** |
| | Min | 0.187 ± 0.015 | 0.713 ± 0.006 | 0.442 ± 0.051 | 0.655 ± 0.012 | 0.118 ± 0.034 | 0.753 ± 0.022 | 17.801 | **0.000** |
| $V-Y$ | Max | 0.578 ± 0.026 | 0.243 ± 0.011 | 0.464 ± 0.082 | 0.274 ± 0.018 | 0.888 ± 0.061 | 0.040 ± 0.038 | 12.995 | **0.000** |
| | Min | 0.322 ± 0.020 | 1.055 ± 0.008 | 0.744 ± 0.058 | 0.969 ± 0.013 | 0.067 ± 0.048 | 1.209 ± 0.030 | 39.595 | **0.000** |
| $V-J$ | Max | 0.634 ± 0.027 | 0.472 ± 0.011 | 0.491 ± 0.082 | 0.511 ± 0.018 | 1.023 ± 0.065 | 0.218 ± 0.041 | 19.620 | **0.000** |
| | Min | 0.373 ± 0.018 | 1.360 ± 0.007 | 0.761 ± 0.054 | 1.281 ± 0.012 | 0.153 ± 0.045 | 1.491 ± 0.028 | 37.602 | **0.000** |
| $V-Ks$ | Max | 0.729 ± 0.027 | 0.782 ± 0.011 | 0.565 ± 0.081 | 0.826 ± 0.018 | 1.156 ± 0.067 | 0.503 ± 0.042 | 24.176 | **0.000** |
| | Min | 0.519 ± 0.016 | 1.686 ± 0.006 | 0.979 ± 0.048 | 1.592 ± 0.010 | 0.252 ± 0.040 | 1.846 ± 0.025 | 67.266 | **0.000** |

**Table 2.** Same as Table 1 but for LMC and SMC FO Cepheids.

| | Phase | $a_{\rm all}$ | $b_{\rm all}$ | $a_{\rm s}$ | $b_{\rm s}$ | $a_{\rm l}$ | $b_{\rm l}$ | $F$ | $p(F)$ |
|---|---|---|---|---|---|---|---|---|---|
| | | | | | LMC | | | | |
| $V-I$ | Max | 0.077 ± 0.007 | 0.451 ± 0.002 | 0.062 ± 0.010 | 0.452 ± 0.002 | 0.265 ± 0.032 | 0.354 ± 0.017 | 10.983 | **0.000** |
| | Min | 0.085 ± 0.006 | 0.595 ± 0.002 | 0.086 ± 0.008 | 0.596 ± 0.002 | 0.200 ± 0.035 | 0.533 ± 0.018 | 5.431 | **0.005** |
| $V-G$ | max | 0.030 ± 0.020 | −0.123 ± 0.007 | 0.043 ± 0.030 | −0.124 ± 0.008 | 0.097 ± 0.084 | −0.162 ± 0.043 | 0.646 | 0.523 |
| | Min | 0.052 ± 0.020 | 0.226 ± 0.007 | 0.089 ± 0.028 | 0.221 ± 0.007 | −0.069 ± 0.090 | 0.282 ± 0.046 | 2.152 | 0.116 |
| $V-Rp$ | Max | 0.115 ± 0.014 | 0.352 ± 0.005 | 0.093 ± 0.020 | 0.354 ± 0.005 | 0.209 ± 0.066 | 0.307 ± 0.034 | 1.752 | 0.174 |
| | Min | 0.079 ± 0.016 | 0.580 ± 0.005 | 0.093 ± 0.022 | 0.578 ± 0.005 | −0.033 ± 0.088 | 0.636 ± 0.046 | 1.154 | 0.315 |
| $V-Y$ | Max | 0.133 ± 0.015 | 0.536 ± 0.005 | 0.119 ± 0.021 | 0.538 ± 0.005 | 0.278 ± 0.071 | 0.463 ± 0.037 | 1.720 | 0.179 |
| | Min | 0.152 ± 0.013 | 0.883 ± 0.004 | 0.168 ± 0.018 | 0.883 ± 0.004 | 0.304 ± 0.078 | 0.795 ± 0.041 | 3.563 | **0.028** |
| $V-J$ | Max | 0.186 ± 0.016 | 0.708 ± 0.005 | 0.188 ± 0.023 | 0.709 ± 0.006 | 0.274 ± 0.080 | 0.660 ± 0.042 | 0.518 | 0.595 |
| | Min | 0.193 ± 0.014 | 1.039 ± 0.005 | 0.212 ± 0.019 | 1.039 ± 0.005 | 0.327 ± 0.080 | 0.960 ± 0.042 | 3.254 | **0.038** |
| $V-Ks$ | Max | 0.239 ± 0.017 | 1.008 ± 0.006 | 0.244 ± 0.024 | 1.010 ± 0.006 | 0.558 ± 0.069 | 0.834 ± 0.036 | 6.676 | **0.000** |
| | Min | 0.252 ± 0.014 | 1.304 ± 0.004 | 0.280 ± 0.0185 | 1.303 ± 0.004 | 0.424 ± 0.078 | 1.201 ± 0.041 | 6.458 | **0.000** |
| | | | | | SMC | | | | |
| $V-I$ | Max | 0.361 ± 0.002 | 0.264 ± 0.009 | 0.361 ± 0.002 | 0.240 ± 0.012 | 0.297 ± 0.040 | 0.420 ± 0.083 | 5.207 | **0.000** |
| | Min | 0.576 ± 0.002 | 0.114 ± 0.007 | 0.576 ± 0.002 | 0.094 ± 0.009 | 0.531 ± 0.042 | 0.228 ± 0.086 | 5.933 | **0.000** |
| $V-G$ | Max | −0.048 ± 0.007 | −0.109 ± 0.001 | −0.041 ± 0.009 | −0.109 ± 0.001 | −0.193 ± 0.058 | −0.040 ± 0.028 | 2.732 | 0.065 |
| | Min | −0.069 ± 0.005 | −0.129 ± 0.001 | −0.066 ± 0.007 | −0.130 ± 0.001 | −0.162 ± 0.046 | −0.085 ± 0.022 | 1.544 | 0.213 |
| $V-Rp$ | Max | 0.394 ± 0.022 | 0.152 ± 0.005 | 0.398 ± 0.029 | 0.153 ± 0.005 | 0.496 ± 0.157 | 0.100 ± 0.076 | 0.146 | 0.863 |
| | Min | 0.091 ± 0.018 | 0.659 ± 0.004 | 0.114 ± 0.023 | 0.659 ± 0.004 | 0.031 ± 0.157 | 0.677 ± 0.076 | 4.816 | 0.319 |
| $V-Y$ | max | 0.381 ± 0.021 | 0.406 ± 0.005 | 0.380 ± 0.028 | 0.407 ± 0.005 | 0.591 ± 0.180 | 0.305 ± 0.087 | 0.429 | 0.650 |
| | Min | 0.182 ± 0.018 | 0.725 ± 0.004 | 0.161 ± 0.024 | 0.726 ± 0.004 | 0.414 ± 0.187 | 0.623 ± 0.090 | 1.505 | 0.222 |
| $V-J$ | Max | 0.488 ± 0.024 | 0.599 ± 0.006 | 0.469 ± 0.033 | 0.600 ± 0.006 | 0.856 ± 0.189 | 0.427 ± 0.092 | 1.510 | 0.221 |
| | Min | 0.182 ± 0.018 | 0.996 ± 0.005 | 0.180 ± 0.025 | 0.997 ± 0.004 | 0.387 ± 0.174 | 0.896 ± 0.085 | 0.655 | 0.519 |
| $V-Ks$ | Max | 0.608 ± 0.027 | 0.852 ± 0.006 | 0.574 ± 0.036 | 0.853 ± 0.006 | 0.897 ± 0.226 | 0.730 ± 0.109 | 1.472 | 0.229 |
| | Min | 0.370 ± 0.019 | 1.283 ± 0.004 | 0.329 ± 0.025 | 1.284 ± 0.004 | 0.709 ± 0.194 | 1.139 ± 0.094 | 4.307 | **0.013** |

**Table 3.** Coefficients of the empirical AC relation for LMC and SMC FU Cepheids at maximum and minimum light assuming a break at $P = 2.5$ d. The bold-face entries indicates the significance of the break.

| | Phase | $a_{\rm all}$ | $b_{\rm all}$ | $a_{\rm s}$ | $b_{\rm s}$ | $a_{\rm l}$ | $b_{\rm l}$ | $F$ | $p(F)$ |
|---|---|---|---|---|---|---|---|---|---|
| | | | | | LMC | | | | |
| $V-I$ | Max | −0.441 ± 0.006 | 0.784 ± 0.005 | −0.376 ± 0.017 | 0.666 ± 0.014 | −0.438 ± 0.006 | 0.790 ± 0.005 | 152.088 | **0.000** |
| | Min | −0.010 ± 0.006 | 0.774 ± 0.005 | 0.048 ± 0.016 | 0.661 ± 0.013 | −0.007 ± 0.006 | 0.779 ± 0.005 | 132.542 | **0.018** |
| $V-G$ | Max | −0.193 ± 0.012 | 0.142 ± 0.009 | −0.265 ± 0.052 | 0.172 ± 0.042 | −0.185 ± 0.012 | 0.138 ± 0.009 | 5.863 | **0.000** |
| | Min | 0.055 ± 0.007 | 0.152 ± 0.005 | 0.072 ± 0.025 | 0.113 ± 0.020 | 0.056 ± 0.007 | 0.153 ± 0.005 | 13.802 | **0.000** |
| $V-Rp$ | Max | −0.387 ± 0.016 | 0.726 ± 0.012 | −0.244 ± 0.071 | 0.588 ± 0.058 | −0.397 ± 0.017 | 0.735 ± 0.011 | 5.220 | **0.000** |
| | Min | 0.079 ± 0.017 | 0.800 ± 0.013 | 0.109 ± 0.052 | 0.687 ± 0.043 | 0.088 ± 0.017 | 0.802 ± 0.013 | 32.485 | **0.000** |
| $V-Y$ | Max | −0.742 ± 0.014 | 1.121 ± 0.011 | −0.768 ± 0.048 | 1.036 ± 0.039 | −0.725 ± 0.014 | 1.120 ± 0.011 | 67.194 | **0.000** |
| | Min | 0.216 ± 0.017 | 0.998 ± 0.013 | 0.225 ± 0.053 | 0.894 ± 0.044 | 0.228 ± 0.017 | 1.000 ± 0.013 | 39.870 | **0.000** |
| $V-J$ | Max | −0.792 ± 0.015 | 1.340 ± 0.012 | −0.771 ± 0.047 | −0.783 ± 0.016 | 1.346 ± 0.012 | 0.307 ± 0.022 | 76.845 | **0.000** |
| | Min | 0.173 ± 0.017 | 1.262 ± 0.014 | 0.207 ± 0.063 | 1.128 ± 0.052 | 0.182 ± 0.018 | 1.268 ± 0.018 | 48.567 | **0.000** |
| $V-Ks$ | Max | −0.904 ± 0.016 | 1.769 ± 0.012 | −0.829 ± 0.047 | 1.551 ± 0.038 | −0.892 ± 0.015 | 1.778 ± 0.012 | 137.245 | **0.000** |
| | Min | 0.135 ± 0.016 | 1.690 ± 0.012 | 0.178 ± 0.053 | 1.496 ± 0.044 | 0.151 ± 0.016 | 1.694 ± 0.012 | 121.051 | **0.000** |
| | | | | | SMC | | | | |
| $V-I$ | Max | −0.388 ± 0.004 | 0.720 ± 0.004 | −0.346 ± 0.005 | 0.656 ± 0.004 | −0.416 ± 0.006 | 0.792 ± 0.005 | 467.944 | **0.000** |
| | Min | 0.052 ± 0.004 | 0.704 ± 0.004 | 0.096 ± 0.005 | 0.642 ± 0.005 | 0.022 ± 0.006 | 0.773 ± 0.006 | 353.510 | **0.000** |
| $V-G$ | Max | −0.150 ± 0.022 | 0.088 ± 0.021 | −0.104 ± 0.037 | 0.024 ± 0.036 | −0.171 ± 0.023 | 0.134 ± 0.020 | 7.459 | **0.000** |
| | Min | 0.050 ± 0.008 | 0.183 ± 0.003 | 0.098 ± 0.030 | 0.170 ± 0.007 | −0.005 ± 0.018 | 0.219 ± 0.011 | 24.867 | **0.000** |
| $V-Rp$ | Max | −0.305 ± 0.020 | 0.615 ± 0.019 | −0.246 ± 0.033 | 0.542 ± 0.031 | −0.343 ± 0.023 | 0.671 ± 0.020 | 8.574 | **0.000** |
| | Min | 0.032 ± 0.011 | 0.761 ± 0.010 | 0.052 ± 0.016 | 0.715 ± 0.015 | 0.051 ± 0.016 | 0.784 ± 0.014 | 44.049 | **0.000** |
| $V-Y$ | Max | −0.733 ± 0.015 | 1.088 ± 0.014 | −0.706 ± 0.019 | 1.010 ± 0.018 | −0.701 ± 0.021 | 1.161 ± 0.019 | 146.766 | **0.000** |
| | Min | 0.237 ± 0.015 | 0.960 ± 0.014 | 0.298 ± 0.019 | 0.854 ± 0.018 | 0.214 ± 0.021 | 1.073 ± 0.019 | 132.871 | **0.000** |
| $V-J$ | Max | −0.812 ± 0.014 | 1.409 ± 0.013 | −0.758 ± 0.017 | 1.302 ± 0.016 | −0.814 ± 0.019 | 1.519 ± 0.017 | 213.275 | **0.000** |
| | Min | 0.215 ± 0.014 | 1.301 ± 0.013 | 0.278 ± 0.017 | 1.191 ± 0.017 | 0.196 ± 0.019 | 1.419 ± 0.017 | 177.161 | **0.000** |
| $V-Ks$ | Max | −0.863 ± 0.013 | 1.788 ± 0.012 | −0.785 ± 0.015 | 1.652 ± 0.014 | −0.890 ± 0.016 | 1.936 ± 0.014 | 24.176 | **0.000** |
| | Min | 0.168 ± 0.015 | 1.725 ± 0.014 | 0.236 ± 0.018 | 1.592 ± 0.017 | 0.165 ± 0.019 | 1.862 ± 0.016 | 67.266 | **0.000** |

**Table 4.** Same as Table 3 but for LMC and SMC FO Cepheids.

| | Phase | $a_{all}$ | $b_{all}$ | $a_s$ | $b_s$ | $a_l$ | $b_l$ | $F$ | $p(F)$ |
|---|---|---|---|---|---|---|---|---|---|
| | | | | | LMC | | | | |
| $V-I$ | Max | −0.375 ± 0.009 | 0.602 ± 0.005 | −0.454 ± 0.011 | 0.625 ± 0.004 | −0.130 ± 0.017 | 0.534 ± 0.005 | 167.161 | **0.000** |
| | Min | 0.044 ± 0.017 | 0.604 ± 0.006 | −0.036 ± 0.019 | 0.628 ± 0.007 | 0.296 ± 0.030 | 0.535 ± 0.010 | 58.298 | **0.018** |
| $V-G$ | Max | −0.137 ± 0.015 | 0.078 ± 0.005 | −0.164 ± 0.018 | 0.086 ± 0.006 | −0.056 ± 0.026 | 0.057 ± 0.009 | 9.024 | **0.000** |
| | Min | 0.065 ± 0.014 | 0.089 ± 0.005 | 0.039 ± 0.016 | 0.096 ± 0.006 | 0.137 ± 0.026 | 0.068 ± 0.009 | 6.706 | **0.000** |
| $V-Rp$ | Max | −0.446 ± 0.032 | 0.596 ± 0.011 | −0.537 ± 0.037 | 0.620 ± 0.013 | −0.207 ± 0.055 | 0.533 ± 0.019 | 20.746 | **0.000** |
| | Min | 0.195 ± 0.030 | 0.592 ± 0.011 | 0.115 ± 0.038 | 0.617 ± 0.013 | 0.395 ± 0.049 | 0.531 ± 0.017 | 10.239 | **0.000** |
| $V-Y$ | Max | −0.682 ± 0.035 | 0.811 ± 0.011 | −0.764 ± 0.041 | 0.832 ± 0.015 | −0.422 ± 0.059 | 0.747 ± 0.020 | 20.348 | **0.000** |
| | Min | 0.321 ± 0.036 | 0.815 ± 0.013 | 0.237 ± 0.042 | 0.835 ± 0.015 | 0.593 ± 0.066 | 0.750 ± 0.023 | 22.221 | **0.000** |
| $V-J$ | Max | −0.720 ± 0.040 | 1.015 ± 0.014 | −0.827 ± 0.047 | 1.042 ± 0.017 | −0.377 ± 0.070 | 0.929 ± 0.024 | 25.231 | **0.000** |
| | Min | 0.275 ± 0.038 | 1.000 ± 0.013 | 0.160 ± 0.045 | 1.029 ± 0.016 | 0.637 ± 0.067 | 0.910 ± 0.023 | 32.171 | **0.000** |
| $V-Ks$ | Max | −0.727 ± 0.041 | 1.355 ± 0.014 | −0.886 ± 0.047 | 1.378 ± 0.017 | −0.231 ± 0.072 | 1.203 ± 0.025 | 44.331 | **0.000** |
| | Min | 0.116 ± 0.039 | 1.337 ± 0.014 | −0.033 ± 0.045 | 1.377 ± 0.016 | 0.589 ± 0.069 | 1.215 ± 0.024 | 46.854 | **0.000** |
| | | | | | SMC | | | | |
| $V-I$ | Max | −0.502 ± 0.010 | 0.630 ± 0.005 | −0.494 ± 0.011 | 0.622 ± 0.005 | −0.214 ± 0.039 | 0.569 ± 0.014 | 65.175 | **0.000** |
| | Min | −0.085 ± 0.010 | 0.631 ± 0.005 | −0.077 ± 0.011 | 0.623 ± 0.005 | 0.189 ± 0.040 | 0.574 ± 0.014 | 57.693 | **0.000** |
| $V-G$ | Max | −0.228 ± 0.012 | 0.104 ± 0.006 | −0.220 ± 0.014 | 0.099 ± 0.006 | −0.166 ± 0.042 | 0.099 ± 0.015 | 6.106 | **0.000** |
| | Min | 0.078 ± 0.010 | 0.100 ± 0.004 | 0.084 ± 0.010 | 0.095 ± 0.005 | 0.130 ± 0.035 | 0.095 ± 0.013 | 6.598 | **0.000** |
| $V-G_{RP}$ | Max | −0.537 ± 0.020 | 0.577 ± 0.010 | −0.514 ± 0.023 | 0.559 ± 0.011 | −0.239 ± 0.074 | 0.530 ± 0.027 | 29.730 | **0.000** |
| | Min | 0.065 ± 0.021 | 0.599 ± 0.010 | 0.068 ± 0.023 | 0.593 ± 0.011 | 0.382 ± 0.074 | 0.521 ± 0.027 | 13.806 | **0.000** |
| $V-Y$ | Max | −0.720 ± 0.025 | 0.798 ± 0.012 | −0.695 ± 0.027 | 0.778 ± 0.013 | −0.445 ± 0.078 | 0.760 ± 0.028 | 20.272 | **0.000** |
| | Min | −0.013 ± 0.024 | 0.760 ± 0.011 | 0.009 ± 0.026 | 0.741 ± 0.013 | 0.263 ± 0.089 | 0.718 ± 0.032 | 20.461 | **0.000** |
| $V-J$ | Max | −0.937 ± 0.028 | 1.116 ± 0.014 | −0.907 ± 0.030 | 1.092 ± 0.015 | −0.469 ± 0.110 | 1.020 ± 0.041 | 33.195 | **0.000** |
| | Min | −0.024 ± 0.028 | 1.042 ± 0.013 | 0.003 ± 0.029 | 1.019 ± 0.015 | 0.422 ± 0.110 | 0.948 ± 0.041 | 30.624 | **0.000** |
| $V-Ks$ | Max | −1.353 ± 0.031 | 1.592 ± 0.015 | −1.279 ± 0.035 | 1.542 ± 0.016 | −1.292 ± 0.214 | 1.671 ± 0.086 | 46.471 | **0.000** |
| | Min | −0.423 ± 0.031 | 1.539 ± 0.016 | −0.352 ± 0.031 | 1.492 ± 0.016 | −0.341 ± 0.225 | 1.610 ± 0.090 | 44.254 | **0.000** |

**Table 5.** Coefficients of the empirical PC relation for the LMC and SMC FU Cepheids at maximum and minimum light assuming a break at $P = 0.58$ d. The bold-face entries indicate the significance of the break.

| | Phase | $a_{all}$ | $b_{all}$ | $a_s$ | $b_s$ | $a_l$ | $b_l$ | $F$ | $p(F)$ | N |
|---|---|---|---|---|---|---|---|---|---|---|
| $V-I$ | Mean | 0.064 ± 0.008 | 0.533 ± 0.002 | 0.134 ± 0.107 | 0.551 ± 0.049 | 0.034 ± 0.012 | 0.540 ± 0.003 | 4.732 | **0.008** | 1017 |
| | Max | 0.076 ± 0.010 | 0.449 ± 0.002 | 0.133 ± 0.100 | 0.457 ± 0.045 | 0.046 ± 0.014 | 0.456 ± 0.004 | 4.176 | 0.015 | - |
| | Min | 0.089 ± 0.008 | 0.595 ± 0.002 | 0.114 ± 0.093 | 0.588 ± 0.042 | 0.057 ± 0.011 | 0.603 ± 0.002 | 7.021 | **0.000** | - |
| $V-Y$ | Max | 0.115 ± 0.021 | 0.538 ± 0.005 | 0.194 ± 0.231 | 0.572 ± 0.104 | 0.110 ± 0.029 | 0.539 ± 0.007 | 0.108 | 0.896 | 967 |
| | Min | 0.168 ± 0.018 | 0.883 ± 0.004 | 0.306 ± 0.163 | 0.913 ± 0.073 | 0.114 ± 0.025 | 0.894 ± 0.006 | 4.484 | **0.011** | - |
| | Mean | 0.119 ± 0.014 | 0.725 ± 0.003 | 0.283 ± 0.165 | 0.766 ± 0.075 | 0.062 ± 0.020 | 0.739 ± 0.004 | 7.886 | **0.000** | - |
| $V-J$ | Max | 0.191 ± 0.023 | 0.709 ± 0.006 | 0.341 ± 0.247 | 0.772 ± 0.111 | 0.182 ± 0.032 | 0.710 ± 0.007 | 0.340 | 0.711 | 967 |
| | Min | 0.212 ± 0.019 | 1.039 ± 0.005 | 0.273 ± 0.196 | 1.036 ± 0.088 | 0.161 ± 0.026 | 1.051 ± 0.006 | 3.562 | **0.028** | - |
| | Mean | 0.114 ± 0.014 | 0.693 ± 0.004 | 0.248 ± 0.169 | 0.718 ± 0.076 | 0.056 ± 0.021 | 0.707 ± 0.004 | 7.427 | **0.000** | - |
| $V-Ks$ | Max | 0.255 ± 0.024 | 1.010 ± 0.006 | 0.337 ± 0.229 | 0.991 ± 0.103 | 0.172 ± 0.033 | 1.030 ± 0.008 | 6.161 | **0.002** | 967 |
| | Min | 0.281 ± 0.018 | 1.301 ± 0.005 | 0.237 ± 0.167 | 1.235 ± 0.075 | 0.213 ± 0.026 | 1.318 ± 0.006 | 7.355 | **0.000** | - |
| | Mean | 0.249 ± 0.021 | 1.176 ± 0.005 | 0.271 ± 0.196 | 1.118 ± 0.088 | 0.147 ± 0.029 | 1.201 ± 0.007 | 12.361 | **0.000** | - |

**Table 6.** Same as Table 5 but for AC relation.

| | Phase | $a_{all}$ | $b_{all}$ | $a_s$ | $b_s$ | $a_l$ | $b_l$ | $F$ | $p(F)$ | N |
|---|---|---|---|---|---|---|---|---|---|---|
| $V-I$ | Max | $-0.422 \pm 0.019$ | $0.609 \pm 0.006$ | $-0.474 \pm 0.068$ | $0.548 \pm 0.020$ | $-0.453 \pm 0.019$ | $0.624 \pm 0.007$ | 56.150 | **0.000** | 1017 |
| | Min | $-0.009 \pm 0.019$ | $0.614 \pm 0.007$ | $-0.043 \pm 0.080$ | $0.556 \pm 0.025$ | $0.035 \pm 0.019$ | $0.627 \pm 0.007$ | 42.416 | **0.000** | - |
| | Mean | $-0.177 \pm 0.019$ | $0.606 \pm 0.007$ | $-0.261 \pm 0.092$ | $0.575 \pm 0.026$ | $-0.206 \pm 0.019$ | $0.620 \pm 0.007$ | 33.201 | **0.000** | - |
| $V-Y$ | Max | $-0.668 \pm 0.034$ | $0.802 \pm 0.012$ | $-0.808 \pm 0.154$ | $0.746 \pm 0.048$ | $-0.762 \pm 0.042$ | $0.811 \pm 0.012$ | 18.459 | **0.000** | 967 |
| | Min | $0.337 \pm 0.035$ | $0.805 \pm 0.012$ | $0.087 \pm 0.169$ | $0.767 \pm 0.052$ | $0.321 \pm 0.042$ | $0.815 \pm 0.013$ | 27.772 | **0.000** | - |
| | Mean | $-0.130 \pm 0.028$ | $0.804 \pm 0.010$ | $-0.398 \pm 0.143$ | $0.779 \pm 0.046$ | $-0.228 \pm 0.032$ | $0.811 \pm 0.010$ | 35.208 | **0.000** | - |
| $V-J$ | Max | $-0.712 \pm 0.039$ | $1.006 \pm 0.014$ | $-1.123 \pm 0.170$ | $0.986 \pm 0.054$ | $-0.824 \pm 0.047$ | $1.015 \pm 0.014$ | 29.877 | **0.000** | 967 |
| | Min | $0.295 \pm 0.038$ | $0.988 \pm 0.013$ | $-0.048 \pm 0.188$ | $0.947 \pm 0.062$ | $0.155 \pm 0.045$ | $0.999 \pm 0.014$ | 37.498 | **0.000** | - |
| | Mean | $-0.138 \pm 0.029$ | $0.773 \pm 0.010$ | $-0.390 \pm 0.148$ | $0.737 \pm 0.048$ | $-0.224 \pm 0.034$ | $0.780 \pm 0.010$ | 32.437 | **0.000** | - |
| $V-Ks$ | Max | $-0.843 \pm 0.049$ | $1.353 \pm 0.017$ | $-1.103 \pm 0.242$ | $1.240 \pm 0.076$ | $-0.893 \pm 0.048$ | $1.381 \pm 0.017$ | 50.102 | **0.000** | 967 |
| | Min | $-0.011 \pm 0.047$ | $1.359 \pm 0.017$ | $-0.329 \pm 0.218$ | $1.290 \pm 0.070$ | $-0.037 \pm 0.046$ | $1.377 \pm 0.016$ | 44.340 | **0.000** | - |
| | Mean | $-0.421 \pm 0.047$ | $1.369 \pm 0.017$ | $-0.789 \pm 0.219$ | $1.293 \pm 0.070$ | $-0.452 \pm 0.045$ | $1.390 \pm 0.016$ | 55.364 | **0.000** | - |

**Table 7.** Same as Table 5 but for PL relation.

| | Phase | $a_{all}$ | $b_{all}$ | $a_s$ | $b_s$ | $a_l$ | $b_l$ | $F$ | $p(F)$ | N |
|---|---|---|---|---|---|---|---|---|---|---|
| $V$ | Max | $-3.279 \pm 0.030$ | $16.541 \pm 0.008$ | $-3.388 \pm 0.303$ | $16.440 \pm 0.138$ | $-3.362 \pm 0.042$ | $16.561 \pm 0.010$ | 3.917 | **0.020** | 1017 |
| | Min | $-3.228 \pm 0.025$ | $16.884 \pm 0.007$ | $-3.398 \pm 0.255$ | $16.747 \pm 0.116$ | $-3.328 \pm 0.036$ | $16.908 \pm 0.009$ | 7.963 | **0.000** | - |
| | Mean | $-3.269 \pm 0.026$ | $16.726 \pm 0.007$ | $-3.545 \pm 0.277$ | $16.540 \pm 0.128$ | $-3.391 \pm 0.039$ | $16.756 \pm 0.010$ | 9.417 | **0.000** | - |
| $I$ | Max | $-3.349 \pm 0.021$ | $16.091 \pm 0.005$ | $-3.483 \pm 0.218$ | $15.994 \pm 0.099$ | $-3.408 \pm 0.029$ | $16.106 \pm 0.007$ | 4.301 | **0.013** | 1017 |
| | Min | $-3.313 \pm 0.018$ | $16.286 \pm 0.005$ | $-3.455 \pm 0.191$ | $16.178 \pm 0.087$ | $-3.387 \pm 0.026$ | $16.304 \pm 0.006$ | 8.215 | **0.000** | - |
| | Mean | $-3.354 \pm 0.019$ | $16.199 \pm 0.005$ | $-3.519 \pm 0.204$ | $16.092 \pm 0.094$ | $-3.417 \pm 0.028$ | $16.214 \pm 0.007$ | 4.918 | **0.007** | - |
| $Y$ | Max | $-3.377 \pm 0.023$ | $16.032 \pm 0.006$ | $-3.276 \pm 0.264$ | $16.031 \pm 0.120$ | $-3.453 \pm 0.032$ | $16.051 \pm 0.006$ | 5.313 | **0.005** | 967 |
| | Min | $-3.380 \pm 0.023$ | $16.032 \pm 0.013$ | $-3.502 \pm 0.235$ | $15.946 \pm 0.106$ | $-3.429 \pm 0.045$ | $16.044 \pm 0.008$ | 2.515 | 0.081 | - |
| | Mean | $-3.367 \pm 0.021$ | $16.029 \pm 0.005$ | $-3.539 \pm 0.148$ | $15.903 \pm 0.102$ | $-3.441 \pm 0.029$ | $16.047 \pm 0.007$ | 7.123 | **0.000** | - |
| $J$ | Max | $-3.448 \pm 0.020$ | $15.822 \pm 0.005$ | $-3.487 \pm 0.207$ | $15.744 \pm 0.093$ | $-3.549 \pm 0.027$ | $15.847 \pm 0.007$ | 12.857 | **0.000** | 967 |
| | Min | $-3.421 \pm 0.020$ | $15.836 \pm 0.005$ | $-3.688 \pm 0.210$ | $15.685 \pm 0.094$ | $-3.470 \pm 0.028$ | $15.848 \pm 0.007$ | 4.535 | **0.010** | - |
| | Mean | $-3.367 \pm 0.021$ | $16.029 \pm 0.005$ | $-3.539 \pm 0.225$ | $15.903 \pm 0.102$ | $-3.441 \pm 0.029$ | $16.047 \pm 0.007$ | 7.123 | **0.000** | - |
| $Ks$ | Max | $-3.516 \pm 0.014$ | $15.473 \pm 0.003$ | $-3.685 \pm 0.149$ | $15.372 \pm 0.066$ | $-3.554 \pm 0.020$ | $15.483 \pm 0.007$ | 5.047 | **0.006** | 967 |
| | Min | $-3.485 \pm 0.015$ | $15.523 \pm 0.005$ | $-3.693 \pm 0.129$ | $15.386 \pm 0.057$ | $-3.549 \pm 0.020$ | $15.539 \pm 0.005$ | 12.621 | **0.000** | - |
| | Mean | $-3.500 \pm 0.014$ | $15.495 \pm 0.004$ | $-3.639 \pm 0.123$ | $15.394 \pm 0.054$ | $-3.557 \pm 0.020$ | $15.509 \pm 0.005$ | 9.516 | **0.000** | - |

**Table 8.** Coefficients of the theoretical PL relation for LMC FO Cepheids using convection sets B and D at mean, maximum and minimum light for the break near to $P = 2.5$ d. The bold-face entries indicates the significance of the break.

| | | Phase | $a_{\rm all}$ | $b_{\rm all}$ | $a_{\rm s}$ | $b_{\rm s}$ | $a_{\rm l}$ | $b_{\rm l}$ | $F$ | $p(F)$ | N |
|---|---|---|---|---|---|---|---|---|---|---|---|
| $V$ | B | Max | $-3.101 \pm 0.035$ | $-2.233 \pm 0.018$ | $-3.064 \pm 0.123$ | $-2.234 \pm 0.027$ | $-3.058 \pm 0.096$ | $-2.262 \pm 0.060$ | 0.180 | 0.835 | 263 |
| | | Min | $-3.252 \pm 0.028$ | $-1.628 \pm 0.016$ | $-3.358 \pm 0.060$ | $-1.613 \pm 0.019$ | $-2.808 \pm 0.110$ | $-1.907 \pm 0.069$ | 10.121 | **0.000** | - |
| | | Mean | $-3.189 \pm 0.029$ | $-1.879 \pm 0.015$ | $-3.397 \pm 0.082$ | $-1.857 \pm 0.018$ | $-2.631 \pm 0.096$ | $-2.227 \pm 0.060$ | 17.150 | **0.000** | - |
| | D | Max | $-2.824 \pm 0.037$ | $-2.202 \pm 0.020$ | $-2.972 \pm 0.133$ | $-2.202 \pm 0.031$ | $-2.869 \pm 0.096$ | $-2.168 \pm 0.060$ | 1.725 | 0.180 | 265 |
| | | Min | $-3.034 \pm 0.029$ | $-1.599 \pm 0.016$ | $-3.308 \pm 0.081$ | $-1.583 \pm 0.019$ | $-2.835 \pm 0.085$ | $-1.717 \pm 0.054$ | 10.609 | **0.000** | - |
| | | Mean | $-2.921 \pm 0.033$ | $-1.882 \pm 0.018$ | $-3.165 \pm 0.107$ | $-1.869 \pm 0.025$ | $-2.726 \pm 0.093$ | $-1.999 \pm 0.058$ | 6.403 | **0.000** | - |
| $I$ | B | Max | $-3.308 \pm 0.025$ | $-2.568 \pm 0.013$ | $-3.369 \pm 0.088$ | $-2.559 \pm 0.019$ | $-3.072 \pm 0.070$ | $-2.717 \pm 0.044$ | 3.194 | **0.042** | 263 |
| | | Min | $-3.419 \pm 0.022$ | $-2.220 \pm 0.011$ | $-3.517 \pm 0.054$ | $-2.205 \pm 0.011$ | $-2.978 \pm 0.082$ | $-2.497 \pm 0.052$ | 15.514 | **0.000** | - |
| | | Mean | $-3.350 \pm 0.023$ | $-2.381 \pm 0.012$ | $-3.527 \pm 0.068$ | $-2.363 \pm 0.014$ | $-2.876 \pm 0.074$ | $-2.677 \pm 0.046$ | 19.479 | **0.000** | - |
| | D | Max | $-3.124 \pm 0.027$ | $-2.573 \pm 0.015$ | $-3.344 \pm 0.092$ | $-2.546 \pm 0.021$ | $-3.043 \pm 0.068$ | $-2.618 \pm 0.042$ | 6.894 | **0.000** | 265 |
| | | Min | $-3.270 \pm 0.025$ | $-2.207 \pm 0.014$ | $-3.536 \pm 0.066$ | $-2.189 \pm 0.015$ | $-3.072 \pm 0.072$ | $-2.326 \pm 0.045$ | 13.954 | **0.000** | - |
| | | Mean | $-3.148 \pm 0.027$ | $-2.404 \pm 0.015$ | $-3.345 \pm 0.093$ | $-2.395 \pm 0.021$ | $-3.011 \pm 0.072$ | $-2.485 \pm 0.045$ | 5.815 | **0.003** | - |
| $G$ | B | Max | $-3.170 \pm 0.031$ | $-2.320 \pm 0.016$ | $-3.149 \pm 0.112$ | $-2.318 \pm 0.025$ | $-3.072 \pm 0.085$ | $-2.384 \pm 0.053$ | 0.406 | 0.666 | 263 |
| | | Min | $-3.295 \pm 0.026$ | $-1.805 \pm 0.014$ | $-3.408 \pm 0.057$ | $-1.788 \pm 0.012$ | $-2.823 \pm 0.103$ | $-2.102 \pm 0.064$ | 13.018 | **0.000** | - |
| | | Mean | $-3.249 \pm 0.027$ | $-2.017 \pm 0.014$ | $-3.450 \pm 0.078$ | $-1.996 \pm 0.017$ | $-2.704 \pm 0.089$ | $-2.358 \pm 0.056$ | 20.527 | **0.000** | - |
| | D | Max | $-2.958 \pm 0.034$ | $-2.283 \pm 0.018$ | $-3.165 \pm 0.115$ | $-2.277 \pm 0.027$ | $-2.936 \pm 0.088$ | $-2.295 \pm 0.055$ | 3.711 | **0.025** | 265 |
| | | Min | $-3.109 \pm 0.026$ | $-1.768 \pm 0.015$ | $-3.381 \pm 0.067$ | $-1.749 \pm 0.015$ | $-2.865 \pm 0.076$ | $-1.916 \pm 0.047$ | 14.851 | **0.000** | - |
| | | Mean | $-2.994 \pm 0.032$ | $-2.031 \pm 0.017$ | $-3.232 \pm 0.101$ | $-2.018 \pm 0.023$ | $-2.803 \pm 0.087$ | $-2.146 \pm 0.054$ | 5.912 | **0.003** | - |
| $G_{RP}$ | B | Max | $-3.312 \pm 0.026$ | $-2.579 \pm 0.014$ | $-3.362 \pm 0.092$ | $-2.573 \pm 0.020$ | $-3.097 \pm 0.073$ | $-2.714 \pm 0.046$ | 2.389 | 0.093 | 263 |
| | | Min | $-3.394 \pm 0.022$ | $-2.217 \pm 0.012$ | $-3.500 \pm 0.054$ | $-2.202 \pm 0.012$ | $-2.935 \pm 0.087$ | $-2.504 \pm 0.055$ | 15.724 | **0.000** | - |
| | | Mean | $-3.335 \pm 0.032$ | $-2.353 \pm 0.017$ | $-3.522 \pm 0.095$ | $-2.331 \pm 0.021$ | $-2.768 \pm 0.106$ | $-2.707 \pm 0.067$ | 19.017 | **0.000** | - |
| | D | Max | $-3.115 \pm 0.028$ | $-2.581 \pm 0.015$ | $-3.330 \pm 0.096$ | $-2.573 \pm 0.022$ | $-3.041 \pm 0.071$ | $-2.622 \pm 0.044$ | 5.993 | **0.002** | 265 |
| | | Min | $-3.234 \pm 0.024$ | $-2.201 \pm 0.013$ | $-3.508 \pm 0.067$ | $-2.184 \pm 0.016$ | $-3.061 \pm 0.068$ | $-2.303 \pm 0.043$ | 15.122 | **0.000** | - |
| | | Mean | $-3.129 \pm 0.028$ | $-2.403 \pm 0.016$ | $-3.343 \pm 0.094$ | $-2.392 \pm 0.022$ | $-2.803 \pm 0.087$ | $-2.146 \pm 0.054$ | 5.252 | **0.005** | - |
| $J$ | B | Max | $-3.432 \pm 0.023$ | $-2.824 \pm 0.012$ | $-3.492 \pm 0.074$ | $-2.813 \pm 0.016$ | $-3.135 \pm 0.062$ | $-3.011 \pm 0.039$ | 6.644 | **0.000** | 263 |
| | | Min | $-3.494 \pm 0.020$ | $-2.623 \pm 0.011$ | $-3.611 \pm 0.054$ | $-2.608 \pm 0.011$ | $-3.091 \pm 0.069$ | $-2.875 \pm 0.043$ | 16.897 | **0.000** | - |
| | | Mean | $-3.459 \pm 0.021$ | $-2.721 \pm 0.011$ | $-3.622 \pm 0.062$ | $-2.703 \pm 0.013$ | $-3.018 \pm 0.065$ | $-2.996 \pm 0.041$ | 18.617 | **0.000** | - |
| | D | Max | $-3.305 \pm 0.023$ | $-2.847 \pm 0.013$ | $-3.509 \pm 0.077$ | $-2.836 \pm 0.018$ | $-3.173 \pm 0.057$ | $-2.925 \pm 0.036$ | 9.086 | **0.000** | 265 |
| | | Min | $-3.717 \pm 0.029$ | $-2.385 \pm 0.016$ | $-4.003 \pm 0.084$ | $-2.360 \pm 0.019$ | $-3.387 \pm 0.077$ | $-2.588 \pm 0.048$ | 16.305 | **0.000** | - |
| | | Mean | $-3.288 \pm 0.024$ | $-2.757 \pm 0.014$ | $-3.467 \pm 0.085$ | $-2.750 \pm 0.019$ | $-3.177 \pm 0.062$ | $-2.822 \pm 0.039$ | 6.899 | **0.000** | - |
| $Ks$ | B | Max | $-3.526 \pm 0.020$ | $-2.973 \pm 0.011$ | $-3.592 \pm 0.066$ | $-2.960 \pm 0.015$ | $-3.167 \pm 0.060$ | $-3.199 \pm 0.038$ | 11.514 | **0.000** | 263 |
| | | Min | $-3.566 \pm 0.019$ | $-2.898 \pm 0.009$ | $-3.698 \pm 0.056$ | $-2.884 \pm 0.013$ | $-3.195 \pm 0.059$ | $-3.130 \pm 0.037$ | 17.799 | **0.000** | - |
| | | Mean | $-3.540 \pm 0.020$ | $-2.946 \pm 0.010$ | $-3.686 \pm 0.060$ | $-2.931 \pm 0.013$ | $-3.140 \pm 0.059$ | $-3.196 \pm 0.037$ | 13.197 | **0.000** | - |
| | D | Max | $-3.440 \pm 0.020$ | $-3.015 \pm 0.011$ | $-3.640 \pm 0.066$ | $-3.001 \pm 0.016$ | $-3.268 \pm 0.052$ | $-3.119 \pm 0.032$ | 12.845 | **0.000** | 265 |
| | | Min | $-3.488 \pm 0.018$ | $-2.911 \pm 0.010$ | $-3.678 \pm 0.056$ | $-2.902 \pm 0.013$ | $-3.406 \pm 0.047$ | $-2.958 \pm 0.029$ | 11.930 | **0.000** | - |
| | | Mean | $-3.404 \pm 0.022$ | $-2.993 \pm 0.013$ | $-3.561 \pm 0.079$ | $-2.987 \pm 0.018$ | $-3.324 \pm 0.049$ | $-3.039 \pm 0.031$ | 6.752 | **0.000** | - |

**Table 9.** Coefficients of the theoretical PC relation for LMC FO Cepheids using convection sets B and D at mean, maximum and minimum light for the break near to $P = 2.5$ d. The bold-face entries indicates the significance of the break.

| | | Phase | $a_{\rm all}$ | $b_{\rm all}$ | $a_{\rm s}$ | $b_{\rm s}$ | $a_{\rm l}$ | $b_{\rm l}$ | $F$ | $p(F)$ | N |
|---|---|---|---|---|---|---|---|---|---|---|---|
| $V-I$ | B | Max | 0.186 ± 0.014 | 0.347 ± 0.007 | 0.257 ± 0.046 | 0.340 ± 0.010 | 0.013 ± 0.037 | 0.454 ± 0.023 | 7.462 | **0.000** | 263 |
| | | Min | 0.172 ± 0.006 | 0.593 ± 0.003 | 0.174 ± 0.013 | 0.595 ± 0.003 | 0.240 ± 0.028 | 0.550 ± 0.017 | 23.551 | **0.000** | - |
| | | Mean | 0.161 ± 0.007 | 0.502 ± 0.004 | 0.131 ± 0.025 | 0.505 ± 0.005 | 0.244 ± 0.029 | 0.450 ± 0.018 | 4.068 | **0.018** | - |
| | D | Max | 0.262 ± 0.012 | 0.391 ± 0.006 | 0.276 ± 0.039 | 0.387 ± 0.009 | 0.177 ± 0.033 | 0.445 ± 0.021 | 2.536 | 0.081 | 265 |
| | | Min | 0.222 ± 0.005 | 0.614 ± 0.003 | 0.196 ± 0.014 | 0.616 ± 0.003 | 0.247 ± 0.019 | 0.599 ± 0.013 | 2.567 | 0.078 | - |
| | | Mean | 0.227 ± 0.008 | 0.522 ± 0.004 | 0.179 ± 0.019 | 0.525 ± 0.004 | 0.285 ± 0.026 | 0.486 ± 0.016 | 5.316 | **0.005** | - |
| $V-G$ | B | Max | 0.070 ± 0.004 | 0.086 ± 0.002 | 0.087 ± 0.013 | 0.084 ± 0.003 | 0.014 ± 0.013 | 0.121 ± 0.008 | 6.865 | **0.000** | 263 |
| | | Min | 0.040 ± 0.002 | 0.178 ± 0.001 | 0.051 ± 0.004 | 0.178 ± 0.001 | 0.046 ± 0.008 | 0.174 ± 0.005 | 3.126 | **0.045** | - |
| | | Mean | 0.053 ± 0.002 | 0.142 ± 0.001 | 0.048 ± 0.009 | 0.143 ± 0.002 | 0.072 ± 0.008 | 0.131 ± 0.005 | 1.647 | 0.194 | - |
| | D | Max | 0.099 ± 0.004 | 0.101 ± 0.002 | 0.099 ± 0.012 | 0.099 ± 0.003 | 0.066 ± 0.011 | 0.122 ± 0.007 | 3.550 | **0.000** | 265 |
| | | Min | 0.058 ± 0.002 | 0.183 ± 0.001 | 0.054 ± 0.004 | 0.183 ± 0.002 | 0.065 ± 0.007 | 0.179 ± 0.004 | 0.852 | 0.427 | - |
| | | Mean | 0.073 ± 0.002 | 0.149 ± 0.002 | 0.067 ± 0.007 | 0.149 ± 0.002 | 0.076 ± 0.007 | 0.147 ± 0.005 | 0.618 | 0.539 | - |
| $V-G_{RP}$ | B | Max | 0.201 ± 0.011 | 0.351 ± 0.006 | 0.273 ± 0.038 | 0.344 ± 0.008 | 0.038 ± 0.032 | 0.452 ± 0.020 | 9.783 | **0.000** | 263 |
| | | Min | 0.141 ± 0.005 | 0.591 ± 0.003 | 0.155 ± 0.012 | 0.592 ± 0.003 | 0.178 ± 0.024 | 0.567 ± 0.015 | 2.058 | 0.129 | - |
| | | Mean | 0.140 ± 0.020 | 0.477 ± 0.010 | 0.127 ± 0.045 | 0.478 ± 0.009 | 0.137 ± 0.084 | 0.480 ± 0.053 | 0.041 | 0.959 | - |
| | D | Max | 0.252 ± 0.010 | 0.400 ± 0.005 | 0.263 ± 0.034 | 0.396 ± 0.008 | 0.175 ± 0.029 | 0.449 ± 0.018 | 2.762 | 0.064 | 265 |
| | | Min | 0.190 ± 0.006 | 0.609 ± 0.003 | 0.168 ± 0.013 | 0.610 ± 0.003 | 0.220 ± 0.020 | 0.591 ± 0.012 | 2.274 | 0.104 | - |
| | | Mean | 0.207 ± 0.007 | 0.521 ± 0.004 | 0.177 ± 0.018 | 0.523 ± 0.004 | 0.245 ± 0.023 | 0.497 ± 0.015 | 2.731 | 0.067 | - |
| $V-J$ | B | Max | 0.334 ± 0.019 | 0.586 ± 0.010 | 0.424 ± 0.061 | 0.576 ± 0.013 | 0.085 ± 0.056 | 0.742 ± 0.035 | 7.582 | **0.000** | 263 |
| | | Min | 0.247 ± 0.011 | 0.997 ± 0.005 | 0.253 ± 0.022 | 0.999 ± 0.005 | 0.331 ± 0.046 | 0.942 ± 0.029 | 2.121 | 0.121 | - |
| | | Mean | 0.263 ± 0.013 | 0.846 ± 0.006 | 0.218 ± 0.040 | 0.851 ± 0.008 | 0.387 ± 0.044 | 0.768 ± 0.028 | 3.691 | **0.026** | - |
| | D | Max | 0.442 ± 0.018 | 0.665 ± 0.010 | 0.443 ± 0.057 | 0.658 ± 0.012 | 0.307 ± 0.052 | 0.751 ± 0.032 | 2.913 | **0.05** | 265 |
| | | Min | 0.652 ± 0.039 | 0.794 ± 0.009 | 0.640 ± 0.114 | 0.789 ± 0.026 | 0.553 ± 0.119 | 0.857 ± 0.075 | 0.357 | 0.700 | - |
| | | Mean | 0.367 ± 0.013 | 0.875 ± 0.007 | 0.302 ± 0.031 | 0.880 ± 0.007 | 0.451 ± 0.041 | 0.823 ± 0.026 | 4.162 | **0.016** | - |
| $V-Ks$ | B | Max | 0.435 ± 0.024 | 0.731 ± 0.013 | 0.541 ± 0.078 | 0.718 ± 0.017 | 0.120 ± 0.074 | 0.928 ± 0.046 | 7.111 | **0.000** | 263 |
| | | Min | 0.329 ± 0.016 | 1.266 ± 0.008 | 0.315 ± 0.037 | 1.270 ± 0.008 | 0.469 ± 0.065 | 1.177 ± 0.041 | 2.588 | 0.077 | - |
| | | Mean | 0.343 ± 0.017 | 1.072 ± 0.009 | 0.280 ± 0.053 | 1.078 ± 0.011 | 0.509 ± 0.059 | 0.968 ± 0.037 | 3.798 | **0.023** | - |
| | D | Max | 0.578 ± 0.023 | 0.832 ± 0.013 | 0.575 ± 0.074 | 0.824 ± 0.017 | 0.401 ± 0.068 | 0.945 ± 0.042 | 2.937 | **0.05** | 265 |
| | | Min | 0.460 ± 0.016 | 1.309 ± 0.009 | 0.354 ± 0.032 | 1.317 ± 0.007 | 0.602 ± 0.056 | 1.222 ± 0.035 | 7.216 | **0.000** | - |
| | | Mean | 0.483 ± 0.017 | 1.110 ± 0.009 | 0.395 ± 0.042 | 1.117 ± 0.009 | 0.597 ± 0.056 | 1.040 ± 0.035 | 4.183 | **0.016** | - |

**Table 10.** Coefficients of the theoretical AC relation for LMC FO Cepheids using convection sets B and D at mean, maximum and minimum light for the break near to $P = 2.5$ d. The bold-face entries indicates the significance of the break.

| | | Phase | $a_{all}$ | $b_{all}$ | $a_s$ | $b_s$ | $a_l$ | $b_l$ | $F$ | $p(F)$ | N |
|---|---|---|---|---|---|---|---|---|---|---|---|
| $V-I$ | B | Max | −0.362 ± 0.021 | 0.621 ± 0.011 | −0.418 ± 0.024 | 0.609 ± 0.014 | −0.170 ± 0.022 | 0.548 ± 0.011 | 115.655 | **0.000** | 263 |
| | | Min | 0.022 ± 0.023 | 0.649 ± 0.013 | −0.041 ± 0.023 | 0.629 ± 0.014 | 0.259 ± 0.021 | 0.561 ± 0.011 | 200.581 | **0.000** | - |
| | | Mean | −0.075 ± 0.022 | 0.613 ± 0.012 | −0.141 ± 0.022 | 0.600 ± 0.013 | 0.148 ± 0.021 | 0.528 ± 0.011 | 98.071 | **0.000** | - |
| | D | Max | −0.473 ± 0.033 | 0.751 ± 0.017 | −0.564 ± 0.041 | 0.734 ± 0.024 | −0.180 ± 0.031 | 0.639 ± 0.014 | 152.637 | **0.000** | 265 |
| | | Min | −0.090 ± 0.033 | 0.762 ± 0.017 | −0.180 ± 0.035 | 0.740 ± 0.020 | 0.223 ± 0.028 | 0.642 ± 0.013 | 224.292 | **0.000** | - |
| | | Mean | −0.198 ± 0.034 | 0.729 ± 0.017 | −0.222 ± 0.036 | 0.669 ± 0.021 | 0.071 ± 0.031 | 0.630 ± 0.014 | 174.454 | **0.000** | - |
| $V-G$ | B | Max | −0.119 ± 0.007 | 0.181 ± 0.004 | −0.128 ± 0.008 | 0.168 ± 0.005 | −0.062 ± 0.008 | 0.161 ± 0.004 | 127.194 | **0.000** | 263 |
| | | Min | 0.001 ± 0.006 | 0.194 ± 0.003 | −0.024 ± 0.007 | 0.196 ± 0.004 | 0.065 ± 0.006 | 0.168 ± 0.003 | 148.898 | **0.000** | - |
| | | Mean | −0.030 ± 0.007 | 0.182 ± 0.004 | −0.050 ± 0.008 | 0.177 ± 0.005 | 0.040 ± 0.006 | 0.155 ± 0.003 | 105.034 | **0.000** | - |
| | D | Max | −0.174 ± 0.011 | 0.236 ± 0.006 | −0.215 ± 0.012 | 0.234 ± 0.007 | −0.060 ± 0.010 | 0.191 ± 0.005 | 203.717 | **0.000** | 265 |
| | | Min | −0.094 ± 0.009 | 0.259 ± 0.005 | −0.067 ± 0.008 | 0.229 ± 0.005 | 0.001 ± 0.014 | 0.219 ± 0.007 | 109.326 | **0.000** | - |
| | | Mean | −0.073 ± 0.010 | 0.220 ± 0.005 | −0.083 ± 0.013 | 0.203 ± 0.007 | 0.012 ± 0.008 | 0.189 ± 0.004 | 180.392 | **0.000** | - |
| $V-G_RP$ | B | Max | −0.335 ± 0.021 | 0.619 ± 0.011 | −0.381 ± 0.023 | 0.598 ± 0.014 | −0.148 ± 0.019 | 0.551 ± 0.010 | 147.505 | **0.000** | 263 |
| | | Min | 0.014 ± 0.020 | 0.640 ± 0.011 | −0.040 ± 0.032 | 0.624 ± 0.013 | 0.212 ± 0.018 | 0.565 ± 0.009 | 178.383 | **0.000** | - |
| | | Mean | 0.032 ± 0.038 | 0.522 ± 0.020 | 0.009 ± 0.044 | 0.486 ± 0.027 | 0.192 ± 0.057 | 0.469 ± 0.029 | 11.024 | **0.000** | - |
| | D | Max | −0.454 ± 0.030 | 0.748 ± 0.016 | −0.577 ± 0.032 | 0.755 ± 0.018 | −0.158 ± 0.027 | 0.632 ± 0.013 | 187.548 | **0.000** | 265 |
| | | Min | −0.291 ± 0.031 | 0.847 ± 0.023 | −0.190 ± 0.025 | 0.741 ± 0.015 | 0.009 ± 0.042 | 0.721 ± 0.020 | 125.053 | **0.000** | - |
| | | Mean | −0.191 ± 0.030 | 0.715 ± 0.015 | −0.216 ± 0.035 | 0.663 ± 0.020 | 0.054 ± 0.027 | 0.625 ± 0.013 | 176.714 | **0.000** | - |
| $V-J$ | B | Max | −0.549 ± 0.035 | 1.028 ± 0.019 | −0.600 ± 0.036 | 0.975 ± 0.022 | −0.265 ± 0.035 | 0.930 ± 0.018 | 143.746 | **0.000** | 263 |
| | | Min | 0.025 ± 0.035 | 1.082 ± 0.019 | −0.068 ± 0.036 | 1.053 ± 0.022 | 0.373 ± 0.032 | 0.952 ± 0.017 | 178.657 | **0.000** | - |
| | | Mean | −0.135 ± 0.035 | 1.033 ± 0.019 | −0.230 ± 0.036 | 1.006 ± 0.022 | 0.211 ± 0.033 | 0.903 ± 0.017 | 105.524 | **0.000** | - |
| | D | Max | −0.783 ± 0.053 | 1.268 ± 0.027 | −0.958 ± 0.055 | 1.257 ± 0.032 | −0.278 ± 0.048 | 1.072 ± 0.023 | 187.837 | **0.000** | 265 |
| | | Min | −0.076 ± 0.126 | 1.133 ± 0.063 | −0.218 ± 0.187 | 0.948 ± 0.106 | 0.828 ± 0.101 | 0.815 ± 0.048 | 138.235 | **0.000** | - |
| | | Mean | −0.331 ± 0.054 | 1.215 ± 0.027 | −0.360 ± 0.061 | 1.114 ± 0.035 | 0.095 ± 0.049 | 1.059 ± 0.023 | 172.870 | **0.000** | - |
| $V-Ks$ | B | Max | −0.707 ± 0.045 | 1.301 ± 0.025 | −0.768 ± 0.047 | 1.229 ± 0.028 | −0.345 ± 0.047 | 1.178 ± 0.024 | 144.821 | **0.000** | 263 |
| | | Min | 0.040 ± 0.047 | 1.380 ± 0.026 | −0.088 ± 0.048 | 1.346 ± 0.026 | 0.503 ± 0.044 | 1.207 ± 0.023 | 172.191 | **0.000** | - |
| | | Mean | −0.173 ± 0.047 | 1.315 ± 0.025 | −0.301 ± 0.048 | 1.281 ± 0.029 | 0.283 ± 0.044 | 1.143 ± 0.022 | 101.889 | **0.000** | - |
| | D | Max | −1.020 ± 0.070 | 1.619 ± 0.060 | −2.234 ± 0.072 | 1.197 ± 0.042 | −0.365 ± 0.064 | 1.365 ± 0.030 | 185.483 | **0.000** | 265 |
| | | Min | −0.146 ± 0.075 | 1.594 ± 0.038 | −0.193 ± 0.081 | 1.458 ± 0.047 | 0.437 ± 0.069 | 1.382 ± 0.032 | 172.613 | **0.000** | - |
| | | Mean | −0.432 ± 0.072 | 1.556 ± 0.036 | −0.473 ± 0.081 | 1.425 ± 0.047 | 0.131 ± 0.066 | 1.350 ± 0.031 | 168.107 | **0.000** | - |

**Table 11.** Coefficients of the theoretical PL relation for SMC FO Cepheids using convection sets B and D at mean, maximum and minimum light assuming for the break near to $P = 2.5$ d. The bold-face entries indicates the significance of the break.

| | | Phase | $a_{\mathrm{all}}$ | $b_{\mathrm{all}}$ | $a_{\mathrm{s}}$ | $b_{\mathrm{s}}$ | $a_{\mathrm{l}}$ | $b_{\mathrm{l}}$ | $F$ | $p(F)$ | N |
|---|---|---|---|---|---|---|---|---|---|---|---|
| $V$ | B | Max | $-3.026 \pm 0.046$ | $-2.308 \pm 0.019$ | $-2.916 \pm 0.089$ | $-2.298 \pm 0.024$ | $-2.699 \pm 0.217$ | $-2.509 \pm 0.131$ | 3.929 | **0.020** | 224 |
| | | Min | $-3.214 \pm 0.039$ | $-1.698 \pm 0.017$ | $-2.980 \pm 0.067$ | $-1.685 \pm 0.017$ | $-2.550 \pm 0.195$ | $-2.106 \pm 0.109$ | 9.788 | **0.000** | - |
| | | Mean | $-3.108 \pm 0.043$ | $-1.968 \pm 0.018$ | $-2.943 \pm 0.070$ | $-1.956 \pm 0.018$ | $-2.724 \pm 0.269$ | $-2.210 \pm 0.149$ | 6.148 | **0.000** | - |
| | D | Max | $-3.070 \pm 0.039$ | $-2.121 \pm 0.017$ | $-3.042 \pm 0.084$ | $-2.122 \pm 0.021$ | $-3.303 \pm 0.197$ | $-1.995 \pm 0.109$ | 0.517 | 0.596 | 233 |
| | | Min | $-2.978 \pm 0.034$ | $-1.652 \pm 0.015$ | $-2.787 \pm 0.070$ | $-1.640 \pm 0.017$ | $-3.170 \pm 0.170$ | $-1.567 \pm 0.094$ | 7.385 | **0.000** | - |
| | | Mean | $-3.029 \pm 0.034$ | $-1.860 \pm 0.015$ | $-2.930 \pm 0.071$ | $-1.853 \pm 0.018$ | $-3.128 \pm 0.178$ | $-1.816 \pm 0.098$ | 1.877 | 0.155 | - |
| $I$ | B | Max | $-3.255 \pm 0.033$ | $-2.635 \pm 0.014$ | $-3.107 \pm 0.064$ | $-2.622 \pm 0.017$ | $-2.690 \pm 0.128$ | $-2.976 \pm 0.071$ | 6.740 | **0.000** | 224 |
| | | Min | $-3.468 \pm 0.030$ | $-2.234 \pm 0.013$ | $-3.304 \pm 0.053$ | $-2.227 \pm 0.013$ | $-2.782 \pm 0.134$ | $-2.643 \pm 0.075$ | 12.785 | **0.000** | - |
| | | Mean | $-3.445 \pm 0.028$ | $-2.388 \pm 0.012$ | $-3.504 \pm 0.041$ | $-2.383 \pm 0.013$ | $-2.137 \pm 0.283$ | $-3.154 \pm 0.169$ | 8.096 | **0.000** | - |
| | D | Max | $-3.224 \pm 0.031$ | $-2.539 \pm 0.013$ | $-3.144 \pm 0.065$ | $-2.536 \pm 0.016$ | $-3.506 \pm 0.167$ | $-2.391 \pm 0.092$ | 2.202 | 0.112 | 233 |
| | | Min | $-3.177 \pm 0.030$ | $-2.256 \pm 0.013$ | $-2.983 \pm 0.062$ | $-2.244 \pm 0.015$ | $-3.477 \pm 0.144$ | $-2.110 \pm 0.079$ | 10.624 | **0.000** | - |
| | | Mean | $-3.190 \pm 0.030$ | $-2.388 \pm 0.013$ | $-3.065 \pm 0.061$ | $-2.381 \pm 0.015$ | $-3.420 \pm 0.157$ | $-2.274 \pm 0.086$ | 4.439 | **0.012** | - |
| $G$ | B | Max | $-3.104 \pm 0.042$ | $-2.391 \pm 0.018$ | $-2.962 \pm 0.082$ | $-2.379 \pm 0.022$ | $-2.629 \pm 0.172$ | $-2.682 \pm 0.095$ | 5.908 | **0.003** | 224 |
| | | Min | $-3.270 \pm 0.037$ | $-1.863 \pm 0.015$ | $-3.050 \pm 0.063$ | $-1.851 \pm 0.016$ | $-2.615 \pm 0.182$ | $-2.266 \pm 0.101$ | 18.719 | **0.000** | - |
| | | Mean | $-3.165 \pm 0.041$ | $-2.102 \pm 0.017$ | $-2.995 \pm 0.066$ | $-2.089 \pm 0.017$ | $-2.822 \pm 0.258$ | $-2.321 \pm 0.143$ | 6.804 | **0.000** | - |
| | D | Max | $-3.142 \pm 0.036$ | $-2.225 \pm 0.016$ | $-3.095 \pm 0.079$ | $-2.224 \pm 0.019$ | $-3.386 \pm 0.185$ | $-2.094 \pm 0.102$ | 0.840 | 0.433 | 233 |
| | | Min | $-3.039 \pm 0.032$ | $-1.828 \pm 0.020$ | $-2.858 \pm 0.066$ | $-1.817 \pm 0.016$ | $-3.248 \pm 0.161$ | $-1.732 \pm 0.089$ | 2.283 | 0.104 | - |
| | | Mean | $-3.089 \pm 0.032$ | $-2.008 \pm 0.014$ | $-2.987 \pm 0.067$ | $-2.002 \pm 0.016$ | $-3.214 \pm 0.171$ | $-1.950 \pm 0.094$ | 6.852 | **0.000** | - |
| $G_{RP}$ | B | Max | $-3.253 \pm 0.034$ | $-2.643 \pm 0.014$ | $-3.110 \pm 0.067$ | $-2.631 \pm 0.017$ | $-2.689 \pm 0.131$ | $-2.983 \pm 0.073$ | 10.289 | **0.000** | 224 |
| | | Min | $-3.349 \pm 0.034$ | $-2.266 \pm 0.014$ | $-3.123 \pm 0.059$ | $-2.253 \pm 0.015$ | $-2.768 \pm 0.155$ | $-2.627 \pm 0.087$ | 21.663 | **0.000** | - |
| | | Mean | $-3.258 \pm 0.038$ | $-2.446 \pm 0.025$ | $-3.078 \pm 0.061$ | $-2.433 \pm 0.016$ | $-2.994 \pm 0.238$ | $-2.623 \pm 0.132$ | 8.227 | **0.000** | - |
| | D | Max | $-3.227 \pm 0.032$ | $-2.537 \pm 0.014$ | $-3.149 \pm 0.067$ | $-2.534 \pm 0.016$ | $-3.508 \pm 0.169$ | $-2.389 \pm 0.093$ | 2.036 | 0.132 | 233 |
| | | Min | $-3.151 \pm 0.030$ | $-2.243 \pm 0.013$ | $-2.986 \pm 0.061$ | $-2.233 \pm 0.015$ | $-3.424 \pm 0.147$ | $-2.111 \pm 0.081$ | 9.365 | **0.000** | - |
| | | Mean | $-3.184 \pm 0.030$ | $-2.380 \pm 0.013$ | $-3.065 \pm 0.061$ | $-2.373 \pm 0.015$ | $-3.391 \pm 0.158$ | $-2.278 \pm 0.087$ | 3.924 | **0.021** | - |
| $J$ | B | Max | $-3.406 \pm 0.030$ | $-2.867 \pm 0.012$ | $-3.224 \pm 0.058$ | $-2.857 \pm 0.015$ | $-2.945 \pm 0.113$ | $-3.153 \pm 0.063$ | 16.860 | **0.000** | 224 |
| | | Min | $-3.461 \pm 0.029$ | $-2.664 \pm 0.012$ | $-3.266 \pm 0.053$ | $-2.653 \pm 0.013$ | $-2.925 \pm 0.130$ | $-2.995 \pm 0.073$ | 21.317 | **0.000** | - |
| | | Mean | $-3.368 \pm 0.035$ | $-2.782 \pm 0.015$ | $-3.177 \pm 0.055$ | $-2.769 \pm 0.014$ | $-3.197 \pm 0.219$ | $-2.909 \pm 0.122$ | 10.415 | **0.000** | - |
| | D | Max | $-3.341 \pm 0.028$ | $-2.829 \pm 0.012$ | $-3.220 \pm 0.057$ | $-2.823 \pm 0.014$ | $-3.673 \pm 0.157$ | $-2.658 \pm 0.086$ | 5.304 | **0.005** | 233 |
| | | Min | $-3.277 \pm 0.027$ | $-2.660 \pm 0.012$ | $-3.093 \pm 0.055$ | $-2.650 \pm 0.014$ | $-3.660 \pm 0.134$ | $-2.466 \pm 0.074$ | 12.384 | **0.000** | - |
| | | Mean | $-3.299 \pm 0.027$ | $-2.745 \pm 0.012$ | $-3.169 \pm 0.055$ | $-2.738 \pm 0.013$ | $-3.583 \pm 0.149$ | $-2.601 \pm 0.082$ | 5.959 | **0.003** | - |
| $Ks$ | B | Max | $-3.419 \pm 0.029$ | $-3.011 \pm 0.012$ | $-3.263 \pm 0.053$ | $-3.000 \pm 0.013$ | $-3.131 \pm 0.106$ | $-3.251 \pm 0.059$ | 27.459 | **0.000** | 224 |
| | | Min | $-3.543 \pm 0.027$ | $-2.932 \pm 0.011$ | $-3.361 \pm 0.050$ | $-2.921 \pm 0.013$ | $-3.048 \pm 0.112$ | $-3.237 \pm 0.062$ | 21.999 | **0.000** | - |
| | | Mean | $-3.448 \pm 0.033$ | $-3.003 \pm 0.014$ | $-3.248 \pm 0.052$ | $-2.990 \pm 0.013$ | $-3.349 \pm 0.204$ | $-3.090 \pm 0.113$ | 12.415 | **0.000** | - |
| | D | Max | $-3.422 \pm 0.027$ | $-3.015 \pm 0.012$ | $-3.269 \pm 0.053$ | $-3.007 \pm 0.013$ | $-3.794 \pm 0.154$ | $-2.824 \pm 0.085$ | 8.767 | **0.000** | 233 |
| | | Min | $-3.373 \pm 0.026$ | $-2.946 \pm 0.011$ | $-3.192 \pm 0.052$ | $-2.936 \pm 0.013$ | $-3.828 \pm 0.130$ | $-2.712 \pm 0.072$ | 14.520 | **0.000** | - |
| | | Mean | $-3.384 \pm 0.026$ | $-2.988 \pm 0.019$ | $-3.244 \pm 0.052$ | $-2.981 \pm 0.013$ | $-3.740 \pm 0.143$ | $-2.805 \pm 0.079$ | 8.189 | **0.000** | - |

**Table 12.** Coefficients of the theoretical PC relation for SMC FO Cepheids using convection sets B and D at mean, maximum and minimum light assuming for the break near to $P = 2.5$ d. The bold-face entries indicates the significance of the break.

| | | Phase | $a_{all}$ | $b_{all}$ | $a_s$ | $b_s$ | $a_l$ | $b_l$ | $F$ | $p(F)$ | N |
|---|---|---|---|---|---|---|---|---|---|---|---|
| $V-I$ | B | Max | 0.188 ± 0.015 | 0.330 ± 0.006 | 0.134 ± 0.031 | 0.329 ± 0.008 | 0.334 ± 0.051 | 0.257 ± 0.029 | 4.525 | **0.011** | 224 |
| | | Min | 0.178 ± 0.006 | 0.571 ± 0.003 | 0.187 ± 0.010 | 0.572 ± 0.003 | 0.217 ± 0.047 | 0.548 ± 0.026 | 1.059 | 0.348 | - |
| | | Mean | 0.156 ± 0.007 | 0.481 ± 0.003 | 0.137 ± 0.017 | 0.481 ± 0.004 | 0.297 ± 0.045 | 0.405 ± 0.025 | 3.886 | **0.021** | - |
| | D | Max | 0.143 ± 0.013 | 0.423 ± 0.006 | 0.089 ± 0.030 | 0.419 ± 0.007 | 0.202 ± 0.058 | 0.396 ± 0.031 | 3.527 | **0.030** | 233 |
| | | Min | 0.202 ± 0.005 | 0.608 ± 0.002 | 0.202 ± 0.010 | 0.608 ± 0.002 | 0.262 ± 0.027 | 0.575 ± 0.015 | 1.719 | 0.181 | - |
| | | Mean | 0.161 ± 0.008 | 0.528 ± 0.004 | 0.134 ± 0.017 | 0.528 ± 0.004 | 0.291 ± 0.041 | 0.458 ± 0.023 | 5.230 | **0.005** | - |
| $V-G$ | B | Max | 0.083 ± 0.004 | 0.073 ± 0.002 | 0.066 ± 0.007 | 0.073 ± 0.002 | 0.136 ± 0.019 | 0.045 ± 0.010 | 6.954 | **0.000** | 224 |
| | | Min | 0.060 ± 0.002 | 0.166 ± 0.001 | 0.075 ± 0.004 | 0.166 ± 0.001 | 0.044 ± 0.012 | 0.172 ± 0.006 | 13.572 | **0.000** | - |
| | | Mean | 0.056 ± 0.004 | 0.134 ± 0.001 | 0.052 ± 0.007 | 0.133 ± 0.002 | 0.098 ± 0.014 | 0.111 ± 0.008 | 2.031 | 0.133 | - |
| | D | Max | 0.061 ± 0.004 | 0.109 ± 0.002 | 0.040 ± 0.010 | 0.108 ± 0.003 | 0.083 ± 0.021 | 0.099 ± 0.012 | 4.306 | **0.014** | 233 |
| | | Min | 0.058 ± 0.002 | 0.178 ± 0.001 | 0.067 ± 0.004 | 0.179 ± 0.001 | 0.059 ± 0.009 | 0.177 ± 0.005 | 4.856 | **0.008** | - |
| | | Mean | 0.059 ± 0.003 | 0.148 ± 0.001 | 0.056 ± 0.006 | 0.147 ± 0.002 | 0.086 ± 0.013 | 0.134 ± 0.006 | 1.211 | 0.299 | - |
| $V-G_{RP}$ | B | Max | 0.231 ± 0.011 | 0.317 ± 0.005 | 0.202 ± 0.024 | 0.317 ± 0.006 | 0.332 ± 0.047 | 0.264 ± 0.026 | 2.370 | 0.095 | 224 |
| | | Min | 0.161 ± 0.006 | 0.562 ± 0.003 | 0.183 ± 0.010 | 0.563 ± 0.003 | 0.166 ± 0.037 | 0.556 ± 0.021 | 3.668 | **0.027** | - |
| | | Mean | 0.149 ± 0.008 | 0.477 ± 0.003 | 0.135 ± 0.014 | 0.478 ± 0.003 | 0.269 ± 0.039 | 0.412 ± 0.022 | 3.542 | **0.030** | - |
| | D | Max | 0.146 ± 0.012 | 0.421 ± 0.005 | 0.095 ± 0.027 | 0.417 ± 0.006 | 0.205 ± 0.053 | 0.394 ± 0.029 | 4.002 | **0.019** | 233 |
| | | Min | 0.170 ± 0.004 | 0.597 ± 0.002 | 0.174 ± 0.009 | 0.597 ± 0.002 | 0.212 ± 0.024 | 0.573 ± 0.013 | 1.368 | 0.256 | - |
| | | Mean | 0.155 ± 0.007 | 0.520 ± 0.003 | 0.134 ± 0.015 | 0.519 ± 0.004 | 0.263 ± 0.041 | 0.462 ± 0.022 | 3.607 | **0.028** | - |
| $V-J$ | B | Max | 0.377 ± 0.019 | 0.542 ± 0.009 | 0.303 ± 0.038 | 0.543 ± 0.010 | 0.608 ± 0.085 | 0.422 ± 0.047 | 5.521 | **0.004** | 224 |
| | | Min | 0.272 ± 0.010 | 0.963 ± 0.005 | 0.313 ± 0.016 | 0.966 ± 0.004 | 0.285 ± 0.064 | 0.949 ± 0.036 | 5.150 | **0.006** | - |
| | | Mean | 0.259 ± 0.014 | 0.814 ± 0.006 | 0.233 ± 0.025 | 0.814 ± 0.006 | 0.472 ± 0.068 | 0.698 ± 0.037 | 3.729 | **0.025** | - |
| | D | Max | 0.260 ± 0.022 | 0.713 ± 0.009 | 0.165 ± 0.047 | 0.707 ± 0.011 | 0.369 ± 0.095 | 0.662 ± 0.051 | 4.541 | **0.011** | 233 |
| | | Min | 0.295 ± 0.008 | 1.018 ± 0.004 | 0.294 ± 0.016 | 1.019 ± 0.004 | 0.422 ± 0.045 | 0.947 ± 0.025 | 3.119 | **0.046** | - |
| | | Mean | 0.270 ± 0.013 | 0.884 ± 0.006 | 0.239 ± 0.028 | 0.884 ± 0.007 | 0.455 ± 0.062 | 0.785 ± 0.030 | 3.527 | **0.031** | - |
| $V-Ks$ | B | Max | 0.409 ± 0.027 | 0.712 ± 0.011 | 0.261 ± 0.051 | 0.708 ± 0.014 | 0.809 ± 0.119 | 0.510 ± 0.062 | 11.548 | **0.000** | 224 |
| | | Min | 0.366 ± 0.016 | 1.225 ± 0.007 | 0.426 ± 0.026 | 1.228 ± 0.006 | 0.377 ± 0.099 | 1.209 ± 0.055 | 4.544 | **0.011** | - |
| | | Mean | 0.339 ± 0.018 | 1.034 ± 0.008 | 0.305 ± 0.034 | 1.035 ± 0.009 | 0.625 ± 0.091 | 0.879 ± 0.050 | 3.765 | **0.024** | - |
| | D | Max | 0.341 ± 0.029 | 0.899 ± 0.012 | 0.214 ± 0.062 | 0.891 ± 0.015 | 0.491 ± 0.126 | 0.829 ± 0.069 | 4.665 | **0.010** | 233 |
| | | Min | 0.390 ± 0.011 | 1.307 ± 0.005 | 0.388 ± 0.022 | 1.309 ± 0.005 | 0.566 ± 0.062 | 1.209 ± 0.034 | 3.210 | **0.042** | - |
| | | Mean | 0.355 ± 0.018 | 1.128 ± 0.008 | 0.314 ± 0.038 | 1.127 ± 0.009 | 0.612 ± 0.083 | 0.989 ± 0.046 | 3.634 | **0.027** | - |

**Table 13.** Coefficients of the theoretical AC relation for SMC FO Cepheids using convection sets B and D at mean, maximum and minimum light assuming for the break near to $P = 2.5$ d. The bold-face entries indicates the significance of the break.

| | | Phase | $a_{all}$ | $b_{all}$ | $a_s$ | $b_s$ $a_l$ $b_l$ | $F$ $p(F)$ | N | | | |
|---|---|---|---|---|---|---|---|---|---|---|---|
| $V-I$ | B | Max | $-0.358 \pm 0.023$ | $0.587 \pm 0.014$ | $-0.351 \pm 0.026$ | $0.547 \pm 0.016$ | $-0.202 \pm 0.026$ | $0.546 \pm 0.014$ | 73.225 | **0.000** | 224 |
| | | Min | $0.039 \pm 0.024$ | $0.599 \pm 0.014$ | $0.047 \pm 0.025$ | $0.556 \pm 0.016$ | $0.209 \pm 0.026$ | $0.555 \pm 0.014$ | 90.129 | **0.000** | - |
| | | Mean | $-0.071 \pm 0.023$ | $0.568 \pm 0.013$ | $-0.071 \pm 0.025$ | $0.534 \pm 0.016$ | $0.095 \pm 0.027$ | $0.519 \pm 0.014$ | 69.742 | **0.000** | - |
| | D | Max | $-0.257 \pm 0.029$ | $0.595 \pm 0.028$ | $-0.290 \pm 0.031$ | $0.566 \pm 0.016$ | $-0.216 \pm 0.032$ | $0.616 \pm 0.016$ | 83.154 | **0.000** | 233 |
| | | Min | $0.144 \pm 0.029$ | $0.592 \pm 0.015$ | $0.105 \pm 0.029$ | $0.561 \pm 0.015$ | $0.199 \pm 0.030$ | $0.611 \pm 0.015$ | 97.256 | **0.000** | - |
| | | Mean | $-0.001 \pm 0.027$ | $0.578 \pm 0.014$ | $-0.029 \pm 0.027$ | $0.548 \pm 0.014$ | $0.031 \pm 0.030$ | $0.603 \pm 0.015$ | 115.413 | **0.000** | - |
| $V-G$ | B | Max | $-0.108 \pm 0.008$ | $0.161 \pm 0.005$ | $-0.095 \pm 0.008$ | $0.140 \pm 0.005$ | $-0.077 \pm 0.010$ | $0.160 \pm 0.005$ | 84.527 | **0.000** | 224 |
| | | Min | $0.013 \pm 0.008$ | $0.175 \pm 0.004$ | $0.017 \pm 0.009$ | $0.161 \pm 0.006$ | $0.060 \pm 0.006$ | $0.163 \pm 0.003$ | 64.428 | **0.000** | - |
| | | Mean | $-0.011 \pm 0.008$ | $0.157 \pm 0.005$ | $-0.004 \pm 0.010$ | $0.140 \pm 0.006$ | $0.027 \pm 0.008$ | $0.151 \pm 0.005$ | 55.888 | **0.000** | - |
| | D | Max | $-0.083 \pm 0.011$ | $0.170 \pm 0.005$ | $-0.092 \pm 0.011$ | $0.155 \pm 0.006$ | $-0.079 \pm 0.012$ | $0.185 \pm 0.006$ | 103.923 | **0.000** | 233 |
| | | Min | $0.044 \pm 0.008$ | $0.173 \pm 0.004$ | $0.035 \pm 0.009$ | $0.164 \pm 0.005$ | $0.058 \pm 0.008$ | $0.178 \pm 0.004$ | 86.166 | **0.000** | - |
| | | Mean | $0.005 \pm 0.009$ | $0.164 \pm 0.005$ | $-0.002 \pm 0.011$ | $0.152 \pm 0.006$ | $0.009 \pm 0.009$ | $0.176 \pm 0.004$ | 90.066 | **0.000** | - |
| $V-G_{RP}$ | B | Max | $-0.324 \pm 0.022$ | $0.575 \pm 0.013$ | $-0.310 \pm 0.024$ | $0.532 \pm 0.015$ | $-0.188 \pm 0.024$ | $0.542 \pm 0.013$ | 83.186 | **0.000** | 224 |
| | | Min | $0.036 \pm 0.021$ | $0.587 \pm 0.013$ | $0.045 \pm 0.024$ | $0.548 \pm 0.015$ | $0.177 \pm 0.021$ | $0.551 \pm 0.011$ | 78.440 | **0.000** | - |
| | | Mean | $-0.055 \pm 0.021$ | $0.554 \pm 0.012$ | $-0.047 \pm 0.023$ | $0.517 \pm 0.014$ | $0.081 \pm 0.024$ | $0.519 \pm 0.012$ | 73.884 | **0.000** | - |
| | D | Max | $-0.223 \pm 0.027$ | $0.578 \pm 0.014$ | $-0.251 \pm 0.029$ | $0.546 \pm 0.015$ | $-0.195 \pm 0.029$ | $0.605 \pm 0.015$ | 96.488 | **0.000** | 233 |
| | | Min | $0.134 \pm 0.025$ | $0.576 \pm 0.013$ | $0.105 \pm 0.027$ | $0.548 \pm 0.014$ | $-0.170 \pm 0.026$ | $0.598 \pm 0.013$ | 103.191 | **0.000** | - |
| | | Mean | $0.005 \pm 0.026$ | $0.565 \pm 0.013$ | $-0.020 \pm 0.027$ | $0.535 \pm 0.014$ | $0.032 \pm 0.029$ | $0.590 \pm 0.015$ | 93.507 | **0.000** | - |
| $V-J$ | B | Max | $-0.525 \pm 0.037$ | $0.961 \pm 0.022$ | $-0.484 \pm 0.038$ | $0.877 \pm 0.023$ | $-0.340 \pm 0.044$ | $0.934 \pm 0.024$ | 88.503 | **0.000** | 224 |
| | | Min | $0.061 \pm 0.037$ | $1.005 \pm 0.022$ | $0.079 \pm 0.042$ | $0.938 \pm 0.026$ | $0.295 \pm 0.036$ | $0.946 \pm 0.019$ | 73.933 | **0.000** | - |
| | | Mean | $-0.088 \pm 0.037$ | $0.941 \pm 0.021$ | $-0.067 \pm 0.041$ | $0.874 \pm 0.025$ | $0.131 \pm 0.041$ | $0.891 \pm 0.022$ | 72.811 | **0.000** | - |
| | D | Max | $-0.387 \pm 0.049$ | $0.986 \pm 0.025$ | $-0.431 \pm 0.051$ | $0.926 \pm 0.026$ | $-0.353 \pm 0.053$ | $1.043 \pm 0.027$ | 99.788 | **0.000** | 233 |
| | | Min | $0.232 \pm 0.044$ | $0.983 \pm 0.023$ | $0.187 \pm 0.046$ | $0.931 \pm 0.024$ | $0.277 \pm 0.048$ | $1.028 \pm 0.024$ | 102.186 | **0.000** | - |
| | | Mean | $0.009 \pm 0.044$ | $0.963 \pm 0.047$ | $-0.031 \pm 0.047$ | $0.910 \pm 0.025$ | $0.044 \pm 0.045$ | $1.012 \pm 0.023$ | 96.247 | **0.000** | - |
| $V-Ks$ | B | Max | $-0.677 \pm 0.048$ | $1.219 \pm 0.028$ | $-0.620 \pm 0.048$ | $1.107 \pm 0.030$ | $-0.447 \pm 0.058$ | $1.189 \pm 0.031$ | 89.538 | **0.000** | 224 |
| | | Min | $0.087 \pm 0.049$ | $1.285 \pm 0.028$ | $0.107 \pm 0.056$ | $1.199 \pm 0.035$ | $0.403 \pm 0.049$ | $1.203 \pm 0.027$ | 72.362 | **0.000** | - |
| | | Mean | $-0.109 \pm 0.049$ | $1.197 \pm 0.028$ | $-0.082 \pm 0.054$ | $1.109 \pm 0.034$ | $0.180 \pm 0.056$ | $1.131 \pm 0.029$ | 71.599 | **0.000** | - |
| | D | Max | $-0.510 \pm 0.065$ | $1.254 \pm 0.033$ | $-0.568 \pm 0.067$ | $1.179 \pm 0.035$ | $-0.466 \pm 0.070$ | $1.334 \pm 0.036$ | 99.103 | **0.000** | 233 |
| | | Min | $0.309 \pm 0.059$ | $1.261 \pm 0.031$ | $0.248 \pm 0.061$ | $1.192 \pm 0.032$ | $0.372 \pm 0.065$ | $1.318 \pm 0.033$ | 99.181 | **0.000** | - |
| | | Mean | $0.010 \pm 0.059$ | $1.232 \pm 0.030$ | $-0.044 \pm 0.063$ | $1.163 \pm 0.033$ | $0.059 \pm 0.061$ | $1.295 \pm 0.031$ | 92.765 | **0.000** | - |

**Table 14.** Coefficients of the PL/PC/AC relation for LMC/SMC FU Cepheids using convection sets B and D at mean, maximum and minimum light. The $F$-test is carried out to test the break near $P$ = 2.5 d.

| | | Phase | $a_{all}$ | $b_{all}$ | $a_s$ | $b_s$ | $a_l$ | $b_l$ | $F$ | $p(F)$ | N |
|---|---|---|---|---|---|---|---|---|---|---|---|
| | | | | | LMC | | | | | | |
| $V$ | B | Max | −2.211 ± 0.111 | −2.391 ± 0.078 | −3.350 ± 0.120 | −2.124 ± 0.027 | −1.042 ± 0.218 | −2.296 ± 0.167 | 36.169 | **0.000** | 197 |
| | | Min | −4.772 ± 0.419 | 2.204 ± 0.298 | −0.0005 ± 0.001 | 0.999 ± 0.001 | −10.102 ± 0.787 | 6.335 ± 0.603 | 42.161 | **0.000** | - |
| | | Mean | −2.228 ± 0.100 | −2.050 ± 0.071 | −3.453 ± 0.080 | −1.803 ± 0.018 | −1.179 ± 0.196 | −2.860 ± 0.196 | 26.179 | **0.000** | - |
| | D | Max | −2.168 ± 0.125 | −2.869 ± 0.091 | −3.894 ± 0.186 | −2.369 ± 0.044 | −1.561 ± 0.175 | −3.342 ± 0.134 | 14.536 | **0.000** | 154 |
| | | Min | −1.954 ± 0.139 | −2.667 ± 0.102 | −3.815 ± 0.145 | −2.057 ± 0.034 | −1.157 ± 0.190 | −3.290 ± 0.146 | 19.550 | **0.000** | - |
| | | Mean | −1.853 ± 0.133 | −2.214 ± 0.097 | −3.740 ± 0.169 | −1.657 ± 0.040 | −1.169 ± 0.185 | −2.748 ± 0.141 | 16.432 | **0.000** | - |
| $I$ | B | Max | −2.462 ± 0.094 | −2.731 ± 0.066 | −3.520 ± 0.090 | −2.500 ± 0.020 | −1.471 ± 0.184 | −3.497 ± 0.141 | 25.378 | **0.000** | 197 |
| | | Min | −2.045 ± 0.129 | −2.817 ± 0.092 | −3.522 ± 0.090 | −2.499 ± 0.020 | −0.677 ± 0.254 | −3.874 ± 0.194 | 25.752 | **0.000** | - |
| | | Mean | −2.465 ± 0.090 | −2.551 ± 0.063 | −3.596 ± 0.072 | −2.324 ± 0.016 | −1.504 ± 0.175 | −3.292 ± 0.134 | 27.762 | **0.000** | - |
| | D | Max | −2.168 ± 0.125 | −2.869 ± 0.091 | −3.894 ± 0.186 | −2.369 ± 0.044 | −1.561 ± 0.175 | −3.342 ± 0.134 | 14.536 | **0.000** | 154 |
| | | Min | −1.954 ± 0.139 | −2.667 ± 0.102 | −3.815 ± 0.145 | −2.057 ± 0.034 | −1.157 ± 0.190 | −3.290 ± 0.146 | 19.550 | **0.000** | - |
| | | Mean | −2.112 ± 0.123 | −2.744 ± 0.090 | −3.845 ± 0.156 | −2.210 ± 0.036 | −1.441 ± 0.169 | −3.268 ± 0.129 | 18.273 | **0.000** | - |
| PC | B | Max | 0.251 ± 0.022 | 0.339 ± 0.015 | 0.169 ± 0.040 | 0.376 ± 0.009 | 0.428 ± 0.046 | 0.201 ± 0.035 | 10.938 | **0.000** | 197 |
| | | Min | −2.727 ± 0.543 | 5.021 ± 0.385 | 3.521 ± 0.090 | 3.498 ± 0.020 | −9.425 ± 1.027 | 10.210 ± 0.786 | 36.234 | **0.000** | - |
| | | Mean | 0.236 ± 0.012 | 0.500 ± 0.008 | 0.143 ± 0.015 | 0.520 ± 0.003 | 0.324 ± 0.026 | 0.432 ± 0.019 | 9.953 | **0.000** | - |
| | D | Max | 0.254 ± 0.426 | 0.426 ± 0.018 | 0.065 ± 0.055 | 0.453 ± 0.013 | 0.265 ± 0.037 | 0.418 ± 0.028 | 1.377 | 0.255 | 154 |
| | | Min | 0.261 ± 0.010 | 0.613 ± 0.007 | 0.165 ± 0.015 | 0.633 ± 0.003 | 0.280 ± 0.016 | 0.599 ± 0.012 | 2.714 | 0.069 | - |
| | | Mean | 0.258 ± 0.014 | 0.529 ± 0.010 | 0.105 ± 0.027 | 0.553 ± 0.006 | 0.271 ± 0.022 | 0.520 ± 0.016 | 2.745 | 0.067 | - |
| AC | B | Max | −0.277 ± 0.042 | 0.675 ± 0.027 | −0.383 ± 0.060 | 0.609 ± 0.034 | −0.316 ± 0.040 | 0.722 ± 0.026 | 36.425 | **0.000** | 197 |
| | | Min | −2.279 ± 0.921 | 4.657 ± 0.593 | 0.420 ± 1.216 | 3.614 ± 0.698 | −2.291 ± 1.032 | 4.580 ± 0.677 | 1.059 | 0.348 | - |
| | | Mean | 0.213 ± 0.032 | 0.581 ± 0.012 | −0.305 ± 0.097 | 0.543*pm*0.034 | 0.231 ± 0.024 | 0.597 ± 0.009 | 94.942 | **0.000** | - |
| | D | Max | −0.114 ± 0.056 | 0.666 ± 0.031 | −0.372 ± 0.125 | 0.661 ± 0.066 | −0.119 ± 0.051 | 0.681 ± 0.028 | 21.818 | **0.000** | 154 |
| | | Min | 0.170 ± 0.039 | 0.702 ± 0.022 | 0.100 ± 0.145 | 0.607 ± 0.077 | 0.162 ± 0.032 | 0.719 ± 0.017 | 47.908 | **0.000** | - |
| | | Mean | 0.215 ± 0.039 | 0.660 ± 0.010 | −0.478 ± 0.213 | 0.676 ± 0.047 | 0.212 ± 0.031 | 0.674 ± 0.008 | 50.480 | **0.000** | - |
| | | | | | SMC | | | | | | |
| $V$ | B | Max | −2.068 ± 0.125 | −2.592 ± 0.091 | −3.225 ± 0.230 | −2.217 ± 0.050 | −0.618 ± 0.220 | −3.710 ± 0.167 | 33.351 | **0.000** | 205 |
| | | Min | −2.040 ± 0.122 | −1.966 ± 0.089 | −3.190 ± 0.143 | −1.596 ± 0.031 | −0.611 ± 0.215 | −3.068 ± 0.144 | 33.443 | **0.000** | - |
| | | Mean | −2.144 ± 0.110 | −2.187 ± 0.080 | −3.284 ± 0.168 | −1.850 ± 0.036 | −0.872 ± 0.193 | −3.165 ± 0.147 | 20.782 | **0.000** | - |
| | D | Max | −2.004 ± 0.118 | −2.565 ± 0.085 | −2.883 ± 0.164 | −2.253 ± 0.040 | −1.236 ± 0.193 | −3.147 ± 0.143 | 13.953 | **0.000** | 192 |
| | | Min | −1.779 ± 0.121 | −2.130 ± 0.087 | −2.488 ± 0.248 | −1.793 ± 0.061 | −0.923 ± 0.193 | −2.779 ± 0.144 | 16.105 | **0.000** | - |
| | | Mean | −2.977 ± 0.052 | −1.854 ± 0.030 | −3.339 ± 0.139 | −1.796 ± 0.039 | −2.823 ± 0.107 | −1.944 ± 0.066 | 5.677 | **0.002** | - |
| $I$ | B | Max | −2.339 ± 0.104 | −2.884 ± 0.076 | −3.389 ± 0.175 | −2.558 ± 0.039 | −1.087 ± 0.182 | −3.849 ± 0.138 | 35.944 | **0.000** | 205 |
| | | Min | −2.306 ± 0.111 | −2.531 ± 0.081 | −3.397 ± 0.137 | −2.188 ± 0.030 | −0.985 ± 0.195 | −3.549 ± 0.148 | 35.064 | **0.000** | - |
| | | Mean | −2.391 ± 0.098 | −2.665 ± 0.071 | −3.434 ± 0.153 | −2.355 ± 0.033 | −1.222 ± 0.170 | −3.564 ± 0.129 | 36.435 | **0.000** | - |
| | D | Max | −2.207 ± 0.101 | −2.973 ± 0.072 | −2.941 ± 0.167 | −2.690 ± 0.041 | −1.504 ± 0.161 | −3.506 ± 0.120 | 16.179 | **0.000** | 192 |
| | | Min | −2.038 ± 0.113 | −2.726 ± 0.081 | −2.714 ± 0.229 | −2.401 ± 0.056 | −1.211 ± 0.179 | −3.353 ± 0.134 | 17.393 | **0.000** | - |
| | | Mean | −3.216 ± 0.043 | −2.368 ± 0.024 | −3.512 ± 0.132 | −2.323 ± 0.037 | −3.106 ± 0.085 | −2.432 ± 0.053 | 5.321 | **0.003** | - |
| PC | B | Max | 0.271 ± 0.028 | 0.291 ± 0.020 | 0.163 ± 0.069 | 0.341 ± 0.015 | 0.469 ± 0.055 | 0.139 ± 0.042 | 9.178 | **0.000** | 205 |
| | | Min | 0.267 ± 0.012 | 0.563 ± 0.009 | 0.207 ± 0.015 | 0.591 ± 0.003 | 0.376 ± 0.023 | 0.479 ± 0.018 | 15.690 | **0.000** | - |
| | | Mean | 0.247 ± 0.015 | 0.478 ± 0.011 | 0.150 ± 0.028 | 0.505 ± 0.006 | 0.349 ± 0.030 | 0.399 ± 0.023 | 8.792 | **0.000** | - |
| | D | Max | 0.202 ± 0.027 | 0.407 ± 0.020 | 0.058 ± 0.050 | 0.437 ± 0.012 | 0.267 ± 0.047 | 0.359 ± 0.035 | 2.182 | 0.115 | 192 |
| | | Min | 0.258 ± 0.010 | 0.596 ± 0.007 | 0.225 ± 0.025 | 0.608 ± 0.006 | 0.288 ± 0.018 | 0.573 ± 0.013 | 2.210 | 0.112 | - |
| | | Mean | 0.241 ± 0.014 | 0.515 ± 0.010 | 0.170 ± 0.028 | 0.526 ± 0.007 | 0.272 ± 0.026 | 0.491 ± 0.019 | 1.834 | 0.162 | - |
| AC | B | Max | −0.353 ± 0.031 | 0.706 ± 0.021 | −0.393 ± 0.074 | 0.600 ± 0.047 | −0.360 ± 0.030 | 0.724 ± 0.023 | 27.538 | **0.000** | 205 |
| | | Min | 0.039 ± 0.026 | 0.722 ± 0.017 | 0.010 ± 0.079 | 0.603 ± 0.050 | 0.031 ± 0.022 | 0.741 ± 0.015 | 51.089 | **0.000** | - |
| | | Mean | 0.232 ± 0.028 | 0.565 ± 0.011 | −0.184 ± 0.065 | 0.592 ± 0.024 | 0.240 ± 0.023 | 0.573 ± 0.009 | 51.551 | **0.000** | - |
| | D | Max | −0.281 ± 0.035 | 0.713 ± 0.021 | −0.109 ± 0.078 | 0.500 ± 0.041 | −0.321 ± 0.033 | 0.747 ± 0.021 | 24.007 | **0.000** | 192 |
| | | Min | 0.033 ± 0.025 | 0.757 ± 0.015 | −0.149 ± 0.133 | 0.751 ± 0.079 | 0.033 ± 0.022 | 0.765 ± 0.014 | 30.324 | **0.000** | - |
| | | Mean | 0.239 ± 0.036 | 0.620 ± 0.010 | 0.313 ± 0.141 | 0.480 ± 0.032 | 0.213 ± 0.031 | 0.637 ± 0.008 | 45.439 | **0.000** | - |

**Table 15.** Comparisons of the PC relation for the FO Cepheids in the LMC. $|T|$ , $p(t)$ represents the observed value and the probability of the $t$-statistics. Bold-faced entries indicate the null hypothesis (equal slopes) can be rejected.

| | Source | $a_{\text{all}}$ | $b_{\text{all}}$ | $\sigma$ | N | Reference | Theoretical/Empirical | $\lvert T\rvert, p(t) w.r.t$ Set B | Set D |
|---|---|---|---|---|---|---|---|---|---|
| $V-I$ | Set B | 0.161 ± 0.007 | 0.502 ± 0.004 | 0.024 | 263 | TW | Theoretical | ... | ... |
| | Set D | 0.227 ± 0.008 | 0.522 ± 0.004 | 0.030 | 265 | TW | Theoretical | **(16.667, 0.000)** | ... |
| | Obs | 0.061 ± 0.006 | 0.534 ± 0.002 | 0.058 | 1355 | TW | Empirical | **(25.819, 0.000)** | **(40.260, 0.000)** |
| $V-G$ | Set B | 0.053 ± 0.002 | 0.142 ± 0.001 | 0.007 | 263 | TW | Theoretical | ... | ... |
| | Set D | 0.073 ± 0.002 | 0.149 ± 0.002 | 0.009 | 265 | TW | Theoretical | **(8.944, 0.000)** | ... |
| | Obs | 0.022 ± 0.005 | 0.066 ± 0.002 | 0.025 | 795 | TW | Empirical | **(6.764,0.000)** | **(12.750,0.000)** |
| $V-G_{RP}$ | Set B | 0.140 ± 0.020 | 0.477 ± 0.010 | 0.102 | 263 | TW | Theoretical | ... | ... |
| | Set D | 0.207 ± 0.007 | 0.521 ± 0.004 | 0.026 | 265 | TW | Theoretical | **(3.576, 0.006)** | ... |
| | Obs | 0.074 ± 0.010 | 0.474 ± 0.003 | 0.059 | 988 | TW | Empirical | **(3.810, 0.005)** | **(18.623, 0.000)** |
| $V-J$ | Set B | 0.263 ± 0.013 | 0.846 ± 0.006 | 0.037 | 263 | TW | Theoretical | ... | ... |
| | Set D | 0.367 ± 0.013 | 0.875 ± 0.007 | 0.048 | 265 | TW | Theoretical | **(20.014, 0.000)** | ... |
| | Obs | 0.123 ± 0.014 | 0.901 ± 0.005 | 0.115 | 1291 | TW | Empirical | **(16.859, 0.000)** | **(24.903, 0.000)** |
| $V-Ks$ | Set B | 0.343 ± 0.017 | 1.072 ± 0.009 | 0.049 | 263 | TW | Theoretical | ... | ... |
| | Set D | 0.483 ± 0.017 | 1.110 ± 0.009 | 0.065 | 265 | TW | Theoretical | **(23.664, 0.000)** | ... |
| | Obs | 0.183 ± 0.017 | 1.181 ± 0.00 | 0.135 | 1291 | TW | Empirical | **(20.000, 0.000)** | **(30.151, 0.190)** |

**Table 16.** Comparisons of the AC relation for the FO Cepheids in the LMC. $|T|$ , $p(t)$ represents the observed value and the probability of the $t$-statistics. Bold-faced entries indicate the null hypothesis (equal slopes) can be rejected.

| | Source | $a_{\text{all}}$ | $b_{\text{all}}$ | $\sigma$ | N | Reference | Theoretical/Empirical | $\lvert T\rvert, p(t) w.r.t$ Set B | Set D |
|---|---|---|---|---|---|---|---|---|---|
| $V-I$ | Set B | −0.075 ± 0.022 | 0.613 ± 0.012 | 0.040 | 263 | TW | Theoretical | ... | ... |
| | Set D | −0.198 ± 0.034 | 0.729 ± 0.028 | 0.053 | 265 | TW | Theoretical | **(4.744, 0.000)** | ... |
| | Obs | −0.109 ± 0.017 | 0.589 ± 0.006 | 0.056 | 1355 | TW | Empirical | **(2.434, 0.007)** | **(3.022, 0.001)** |
| $V-G$ | Set B | −0.030 ± 0.007 | 0.182 ± 0.004 | 0.012 | 263 | TW | Theoretical | ... | ... |
| | Set D | −0.073 ± 0.010 | 0.220 ± 0.005 | 0.015 | 265 | TW | Theoretical | **(6.021, 0.000)** | ... |
| | Obs | −0.025 ± 0.010 | 0.082 ± 0.004 | 0.025 | 795 | TW | Empirical | (0.589, 0.227) | **(10.474, 0.000)** |
| $V-G_{RP}$ | Set B | 0.032 ± 0.038 | 0.522 ± 0.020 | 0.098 | 263 | TW | Theoretical | ... | ... |
| | Set D | −0.191 ± 0.030 | 0.715 ± 0.015 | 0.047 | 265 | TW | Theoretical | **(9.561, 0.000)** | ... |
| | Obs | −0.100 ± 0.022 | 0.530 ± 0.008 | 0.060 | 988 | TW | Empirical | **(4.260, 0.000)** | **(4.461, 0.001)** |
| $V-J$ | Set B | −0.135 ± 0.035 | 1.033 ± 0.019 | 0.064 | 263 | TW | Theoretical | ... | ... |
| | Set D | −0.331 ± 0.054 | 1.215 ± 0.027 | 0.084 | 265 | TW | Theoretical | **(4.766, 0.000)** | ... |
| | Obs | −0.138 ± 0.029 | 0.773 ± 0.010 | 0.095 | 1291 | TW | Empirical | (0.153, 0.439) | **(4.236, 0.000)** |
| $V-Ks$ | Set B | −0.173 ± 0.047 | 1.315 ± 0.025 | 0.084 | 263 | TW | Theoretical | ... | ... |
| | Set D | −0.432 ± 0.072 | 1.556 ± 0.036 | 0.113 | 265 | TW | Theoretical | **(4.748, 0.000)** | ... |
| | Obs | −0.255 ± 0.041 | 1.329 ± 0.014 | 0.127 | 1291 | TW | Empirical | **(3.568, 0.000)** | **(2.990, 0.001)** |

**Table 17.** Comparisons of the PC relation for the FO Cepheids in the SMC. $|T|$ , $p(t)$ represents the observed value and the probability of the $t$-statistics. Bold-faced entries indicate the null hypothesis (equal slopes) can be rejected.

| | Source | $a_{\rm all}$ | $b_{\rm all}$ | $\sigma$ | N | Reference | Theoretical/Empirical | $\|T\|, p(t) w.r.t$ Set B | Set D |
|---|---|---|---|---|---|---|---|---|---|
| $V-I$ | Set B | 0.156 ± 0.007 | 0.486 ± 0.003 | 0.026 | 224 | TW | Theoretical | ... | ... |
| | Set D | 0.161 ± 0.008 | 0.528 ± 0.004 | 0.026 | 233 | TW | Theoretical | (1.212, 0.113) | ... |
| | Obs | 0.160 ± 0.007 | 0.485 ± 0.002 | 0.062 | 1532 | TW | Empirical | (0.707, 0.239) | (0.258, 0.398) |
| $V-G$ | Set B | 0.056 ± 0.004 | 0.134 ± 0.001 | 0.008 | 224 | TW | Theoretical | ... | ... |
| | Set D | 0.059 ± 0.003 | 0.148 ± 0.001 | 0.008 | 233 | TW | Theoretical | (1.341, 0.090) | ... |
| | Obs | 0.040 ± 0.004 | 0.064 ± 0.001 | 0.028 | 1182 | TW | Empirical | **(6.047, 0.000)** | **(5.484, 0.000)** |
| $V-G_{RP}$ | Set B | 0.149 ± 0.008 | 0.477 ± 0.003 | 0.023 | 224 | TW | Theoretical | ... | ... |
| | Set D | 0.155 ± 0.007 | 0.520 ± 0.003 | 0.026 | 233 | TW | Theoretical | (1.549, 0.061) | ... |
| | Obs | 0.164 ± 0.010 | 0.421 ± 0.002 | 0.068 | 1162 | *TW* | Empirical | **(2.100, 0.017)** | (1.500, 0.060) |
| $V-Y$ | Set B | 0.259 ± 0.014 | 0.814 ± 0.006 | 0.039 | 224 | TW | Theoretical | ... | ... |
| | Set D | 0.270 ± 0.013 | 0.884 ± 0.006 | 0.040 | 233 | *TW* | Theoretical | (1.469, 0.071) | ... |
| | Obs | 0.223 ± 0.014 | 0.625 ± 0.003 | 0.132 | 1425 | TW | Empirical | **(6.928, 0.000)** | **(8.727, 0.000)** |
| $V-Ks$ | Set B | 0.339 ± 0.018 | 1.034 ± 0.008 | 0.053 | 224 | TW | Theoretical | ... | ... |
| | Set D | 0.355 ± 0.018 | 1.128 ± 0.008 | 0.055 | 233 | TW | Theoretical | **(2.708, 0.003)** | ... |
| | Obs | 0.409 ± 0.019 | 1.068 ± 0.004 | 0.147 | 1425 | TW | Empirical | **(11.507, 0.000)** | **(6.363, 0.000)** |

**Table 18.** Comparisons of the AC relation for the FO Cepheids in the SMC. $|T|$ , $p(t)$ represents the observed value and the probability of the $t$-statistics. Bold-faced entries indicate the null hypothesis (equal slopes) can be rejected.

| | Source | $a_{\rm all}$ | $b_{\rm all}$ | $\sigma$ | N | Reference | Theoretical/Empirical | $\|T\|, p(t) w.r.t$ Set B | Set D |
|---|---|---|---|---|---|---|---|---|---|
| $V-I$ | Set B | −0.071 ± 0.023 | 0.568 ± 0.013 | 0.046 | 224 | TW | Theoretical | ... | ... |
| | Set D | −0.001 ± 0.027 | 0.578 ± 0.014 | 0.052 | 233 | TW | Theoretical | **(4.949, 0.000)** | ... |
| | Obs | −0.236 ± 0.010 | 0.618 ± 0.005 | 0.057 | 1532 | TW | Empirical | **(7.966, 0.000)** | **(9.370,0.000)** |
| $V-G$ | Set B | −0.011 ± 0.008 | 0.174 ± 0.005 | 0.017 | 224 | TW | Theoretical | ... | ... |
| | Set D | −0.001 ± 0.019 | 0.173 ± 0.010 | 0.018 | 233 | TW | Theoretical | (0.580, 0.281) | ... |
| | Obs | −0.046 ± 0.005 | 0.090 ± 0.002 | 0.028 | 1182 | TW | Empirical | **(5.604, 0.000)** | **(2.454, 0.007)** |
| $V-G_{RP}$ | Set B | −0.055 ± 0.021 | 0.554 ± 0.012 | 0.044 | 224 | TW | Theoretical | ... | ... |
| | Set D | 0.005 ± 0.025 | 0.565 ± 0.013 | 0.051 | 233 | TW | Theoretical | **(4.423, 0.000)** | ... |
| | Obs | −0.175 ± 0.014 | 0.526 ± 0.007 | 0.071 | 1162 | TW | Empirical | **(7.666, 0.000)** | **(8.690, 0.000)** |
| $V-J$ | Set B | −0.088 ± 0.037 | 0.941 ± 0.021 | 0.076 | 224 | TW | Theoretical | ... | ... |
| | Set D | 0.009 ± 0.044 | 0.963 ± 0.047 | 0.087 | 233 | TW | Theoretical | **(4.073, 0.000)** | ... |
| | Obs | −0.370 ± 0.023 | 1.052 ± 0.010 | 0.138 | 1425 | TW | Empirical | **(9.729, 0.000)** | **(10.103, 0.000)** |
| $V-Ks$ | Set B | −0.109 ± 0.049 | 1.197 ± 0.028 | 0.101 | 224 | TW | Theoretical | ... | ... |
| | Set D | 0.010 ± 0.059 | 1.232 ± 0.030 | 0.114 | 233 | TW | Theoretical | **(3.621, 0.000)** | ... |
| | Obs | −0.508 ± 0.028 | 1.358 ± 0.013 | 0.155 | 1425 | TW | Empirical | **(9.922, 0.000)** | **(9.974, 0.000)** |
